# Supplementary material for: What is being transferred in transfer learning?
Source: arXiv:2008.11687 ancillary file (2021-01-14)
Supplement: Supplementary file 1 [file criticality-plots.pdf]

# Supplementary Material for 'What is being transferred in transfer learning?' Criticality plots for Chexpert

Behnam Neyshabur*
Google
neyshabur@google.com

Hanie Sedghi*
Google Brain
hsedghi@google.com

Chiyuan Zhang*
Google Brain
chiyuan@google.com

*Equal contribution. Authors ordered randomly.

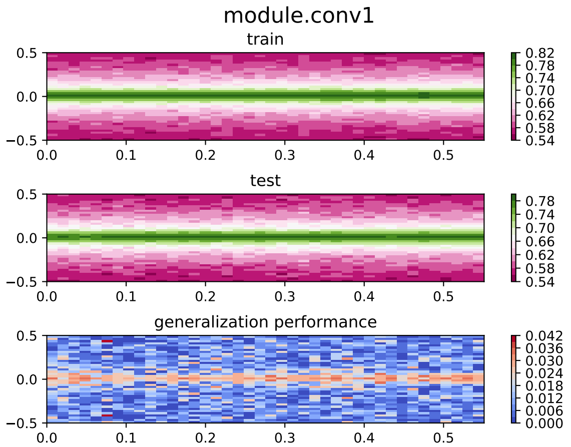


(a) P-T, direct path

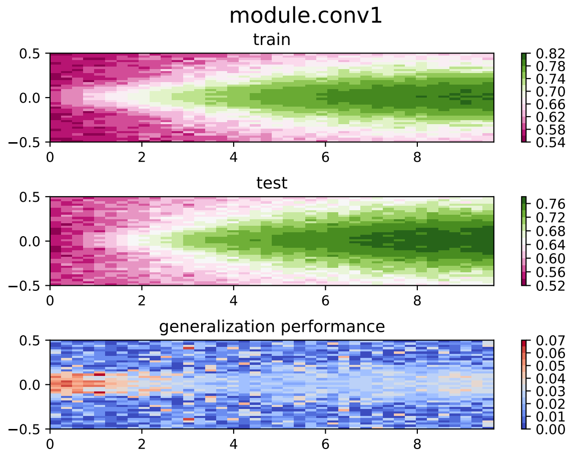


(b) RI-T, direct path

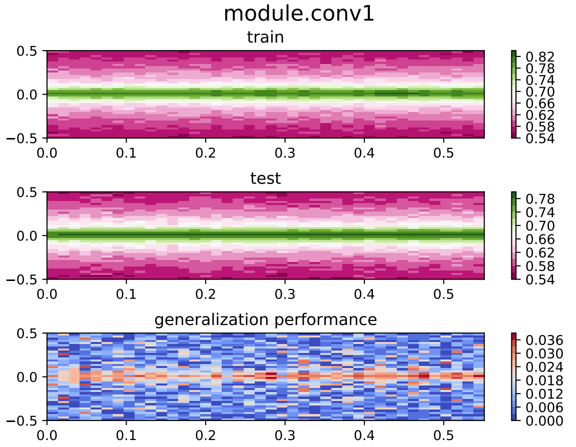


(c) P-T, optimization path

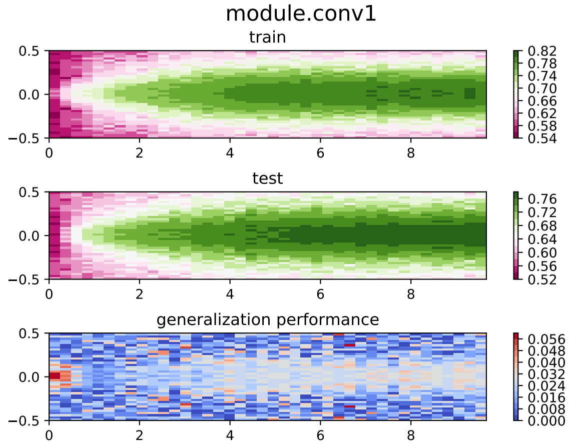


(d) RI-T, optimization path

Figure 1: **Module Criticality Conv1**

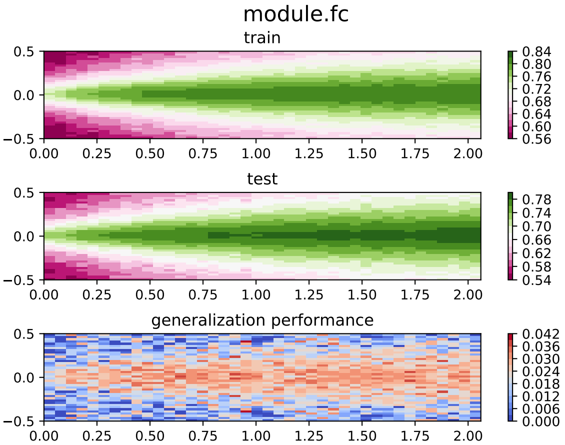


(a) P-T, direct path

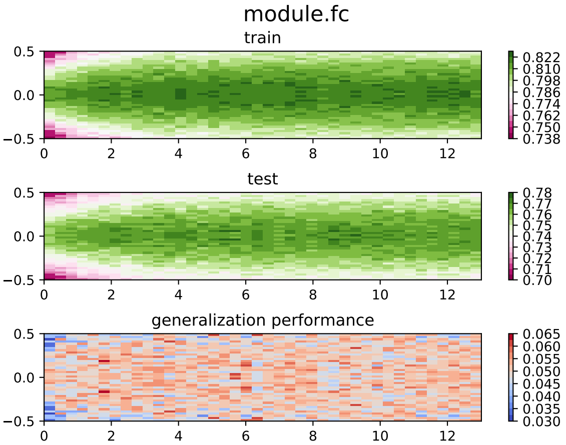


(b) RI-T, direct path

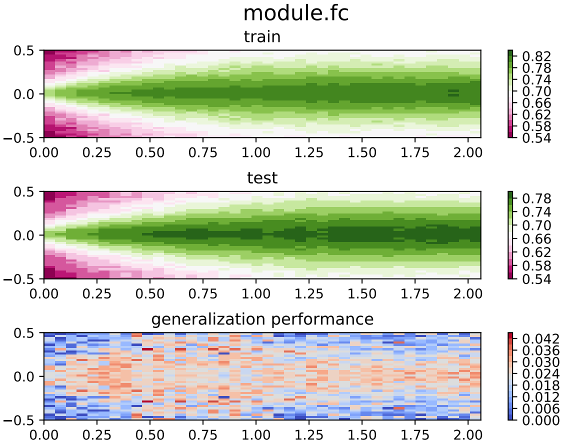


(c) P-T, optimization path

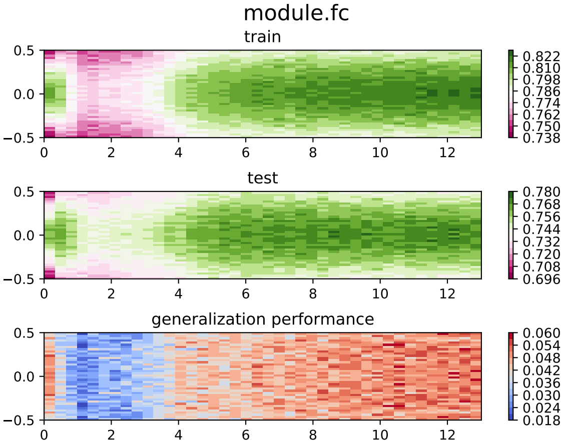


(d) RI-T, optimization path

Figure 2: **Module Criticality FC**

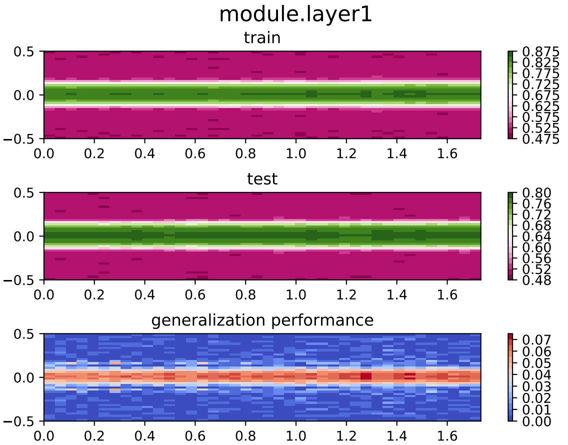


(a) P-T, direct path

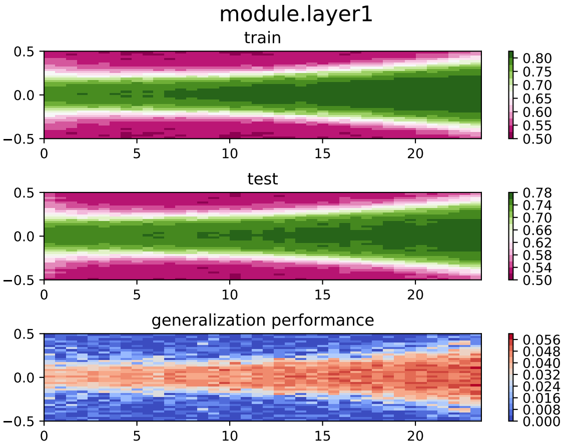


(b) RI-T, direct path

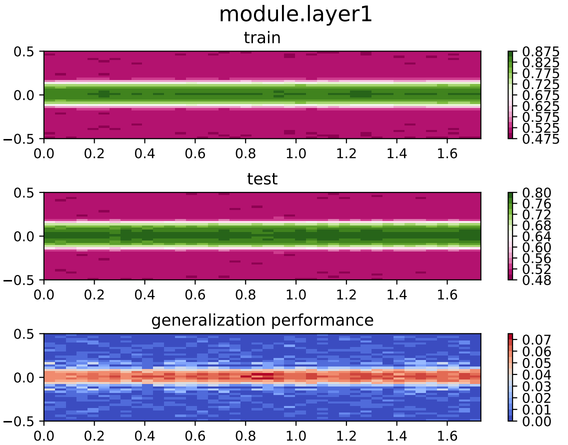


(c) P-T, optimization path

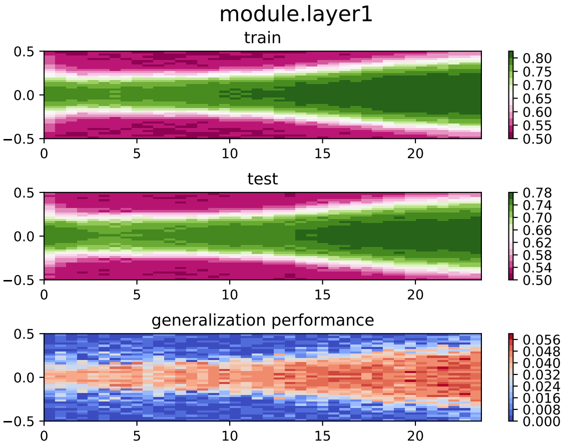


(d) RI-T, optimization path

Figure 3: **Module Criticality Layer1**

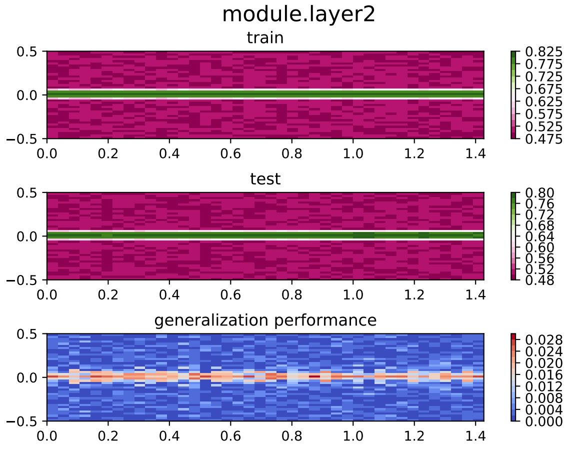


(a) P-T, direct path

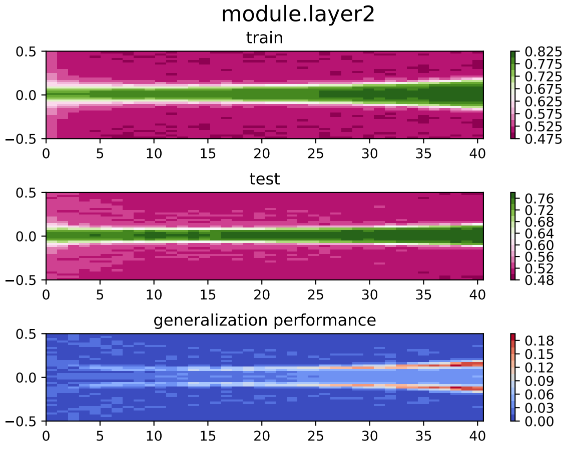


(b) RI-T, direct path

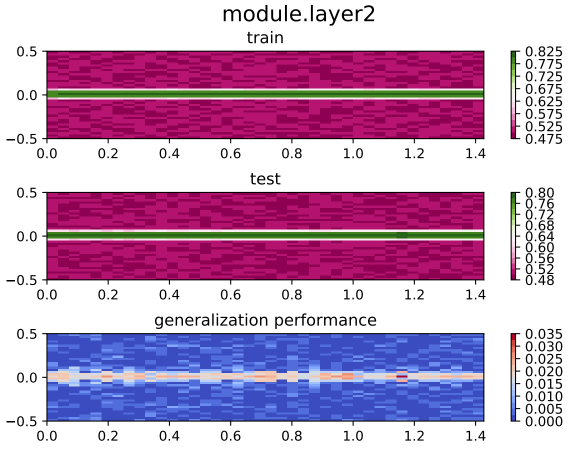


(c) P-T, optimization path

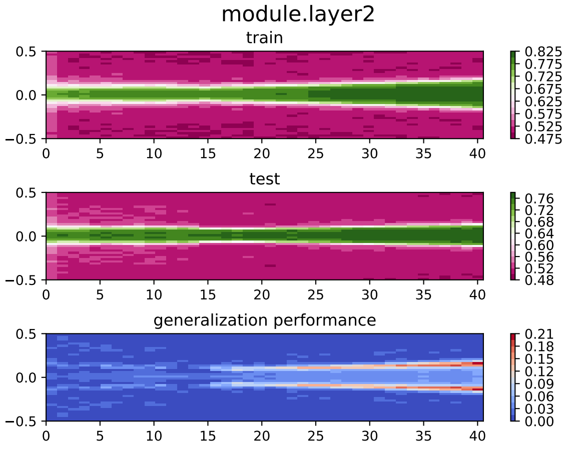


(d) RI-T, optimization path

Figure 4: **Module Criticality Layer2**

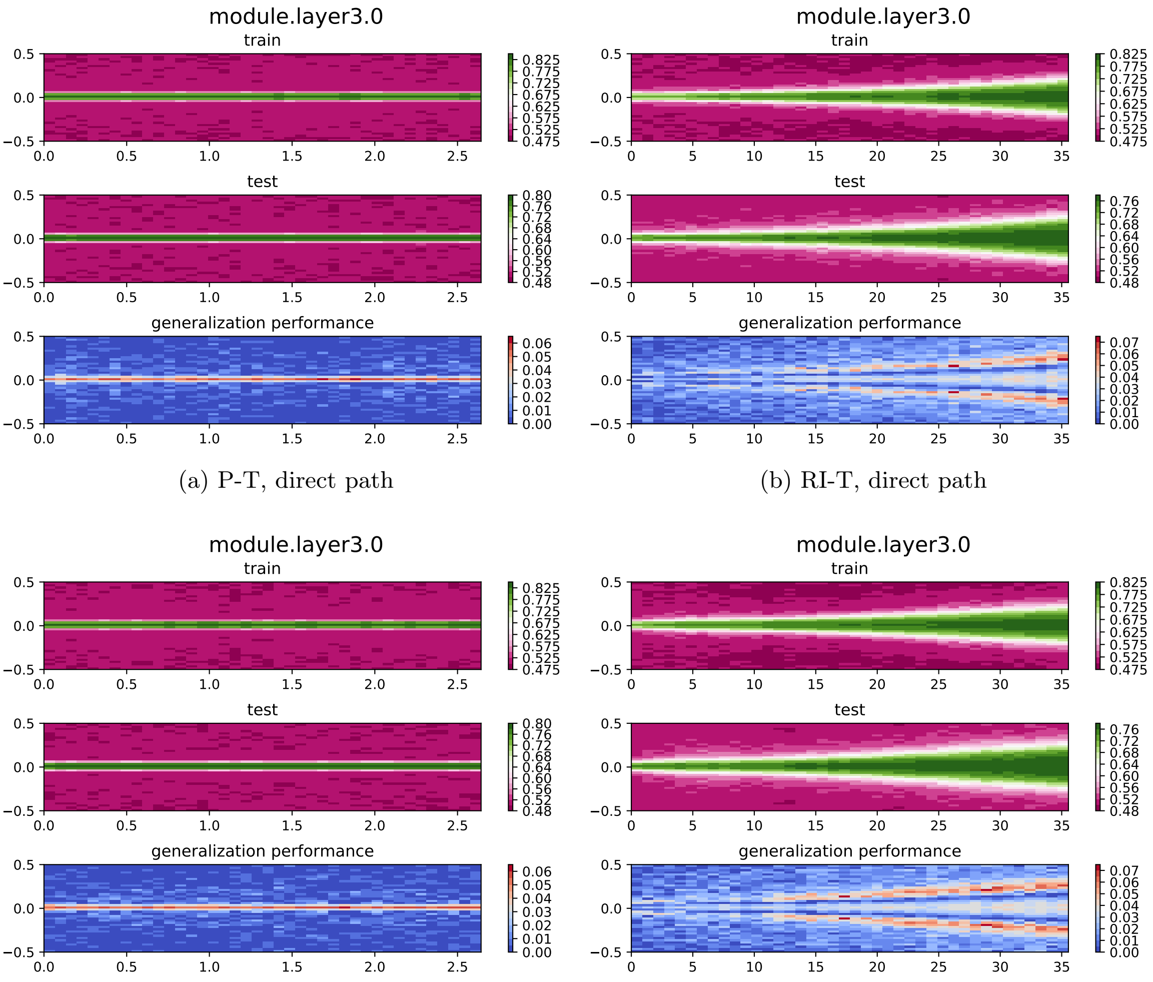


(a) P-T, direct path

(b) RI-T, direct path

(c) P-T, optimization path

(d) RI-T, optimization path

Figure 5: **Module Criticality Layer3.0**

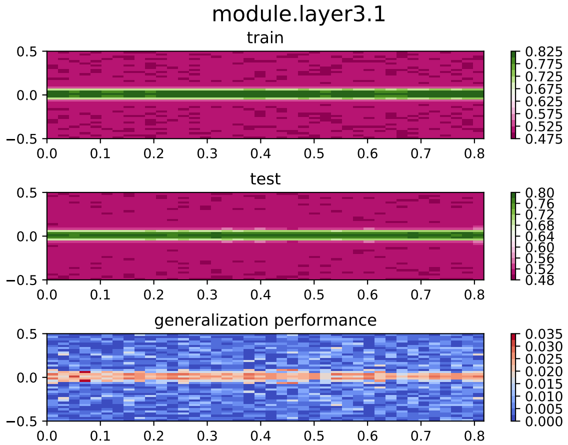


(a) P-T, direct path

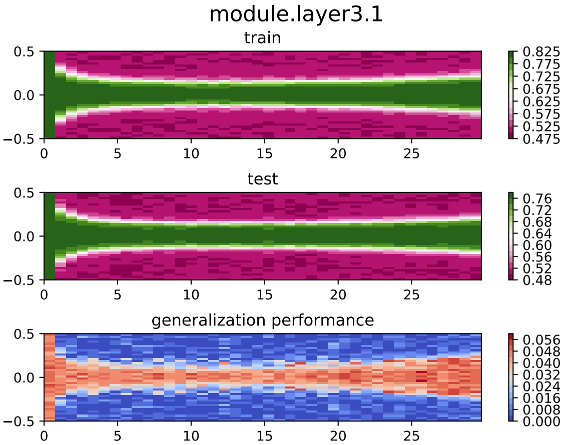


(b) RI-T, direct path

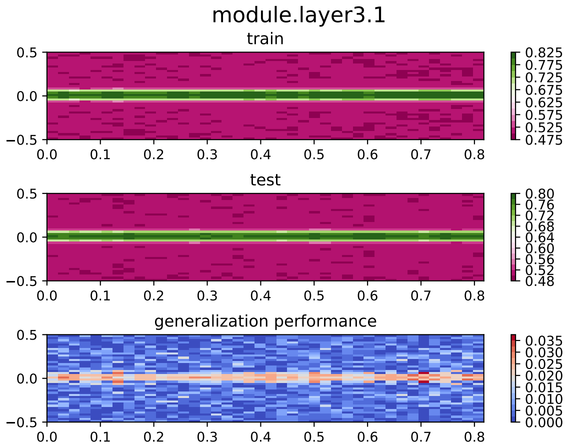


(c) P-T, optimization path

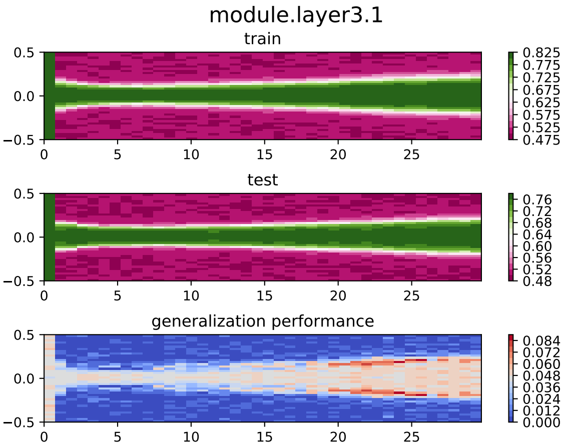


(d) RI-T, optimization path

Figure 6: **Module Criticality Layer3.1**

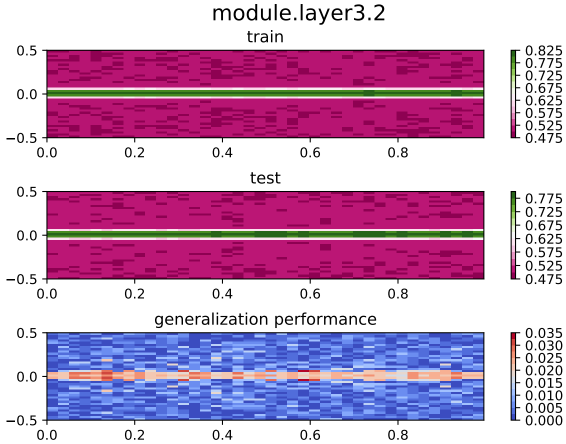


(a) P-T, direct path

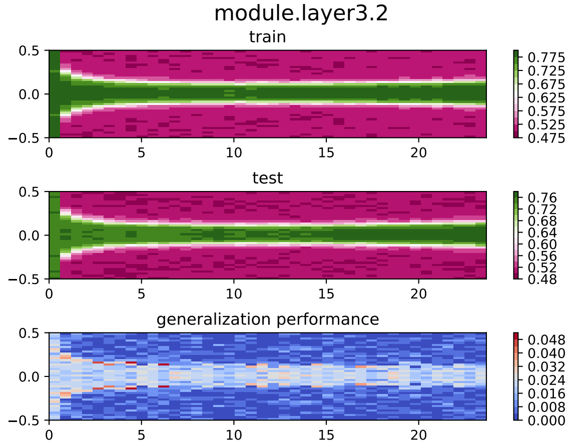


(b) RI-T, direct path

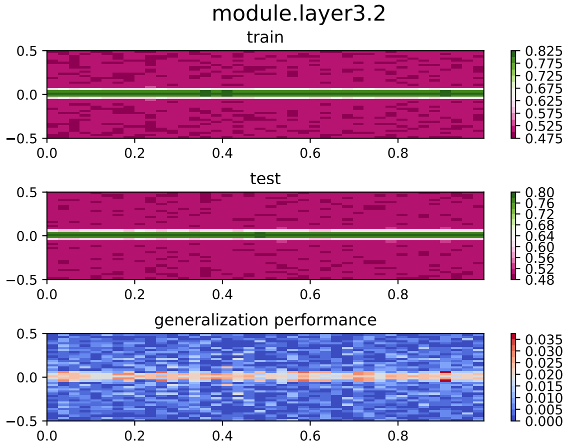


(c) P-T, optimization path

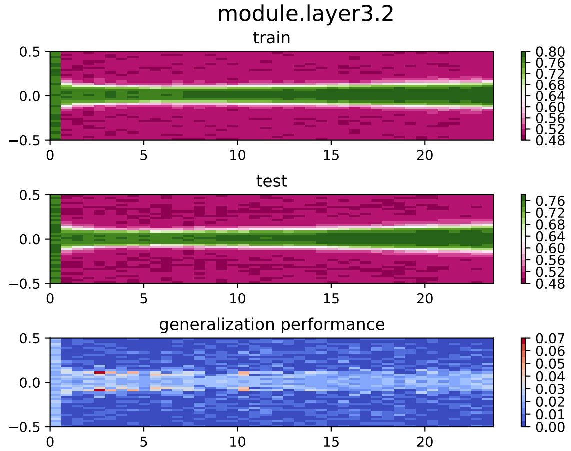


(d) RI-T, optimization path

Figure 7: **Module Criticality Layer3.2**

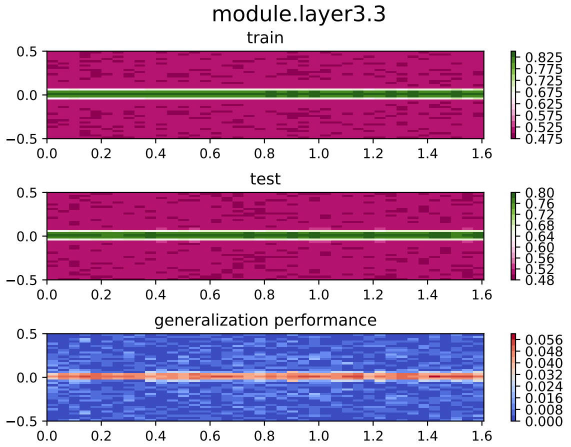


(a) P-T, direct path

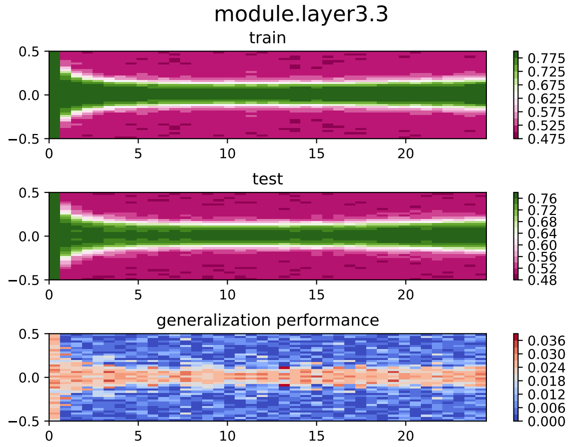


(b) RI-T, direct path

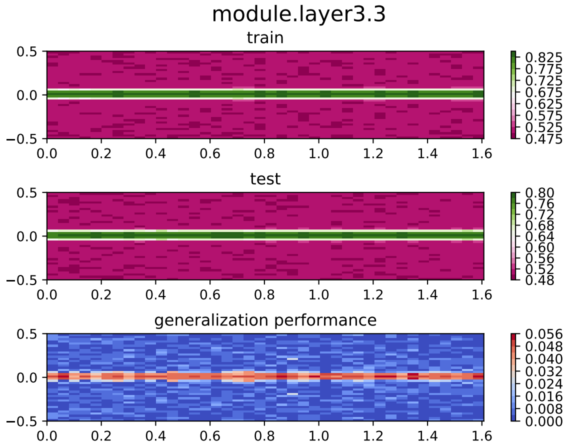


(c) P-T, optimization path

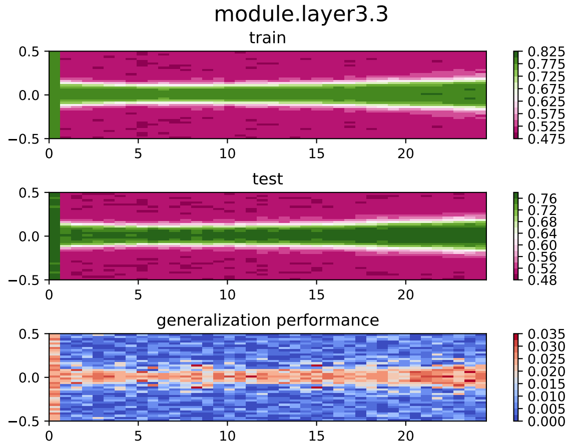


(d) RI-T, optimization path

Figure 8: **Module Criticality Layer3.3**

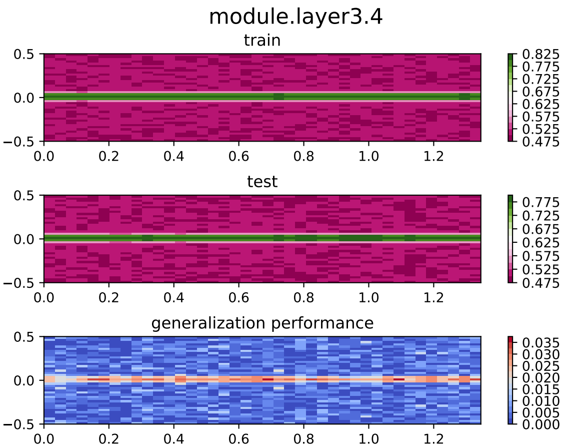


(a) P-T, direct path

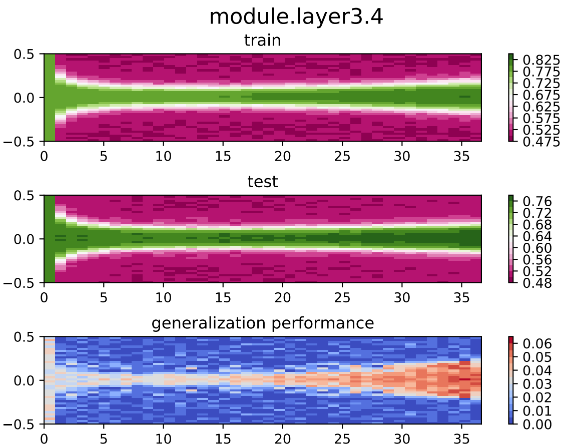


(b) RI-T, direct path

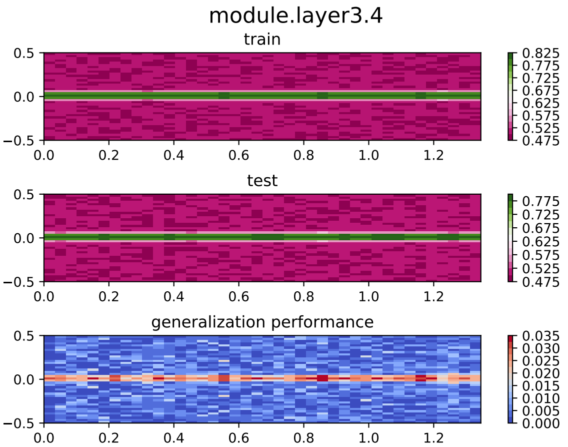


(c) P-T, optimization path

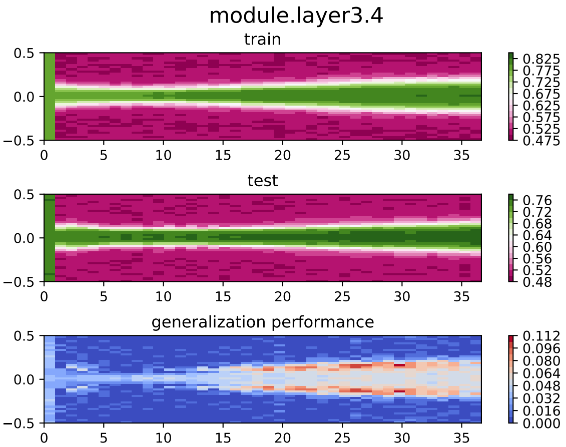


(d) RI-T, optimization path

Figure 9: **Module Criticality Layer3.4**

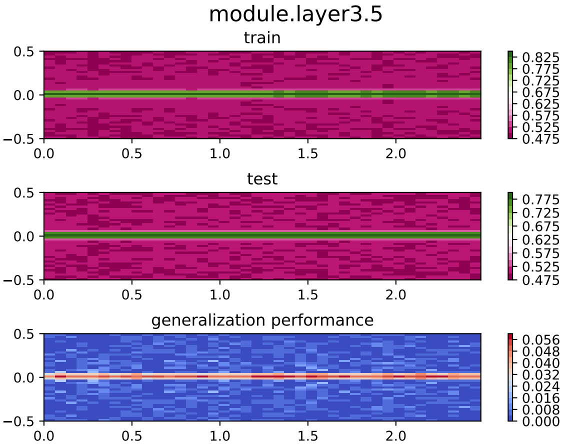


(a) P-T, direct path

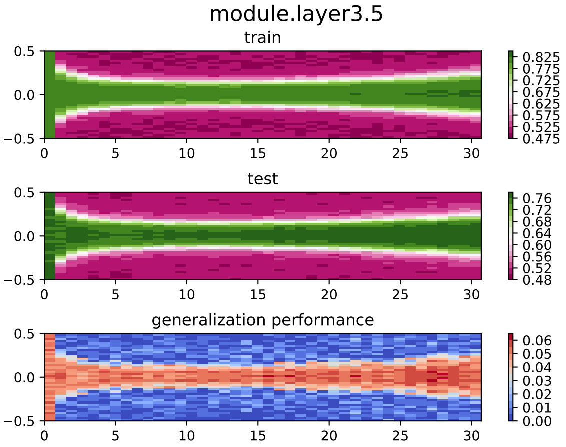


(b) RI-T, direct path

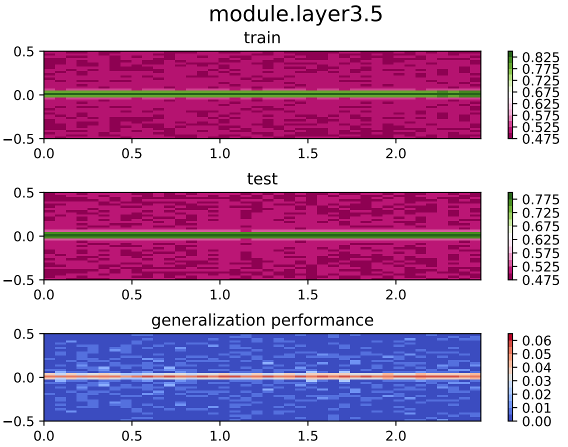


(c) P-T, optimization path

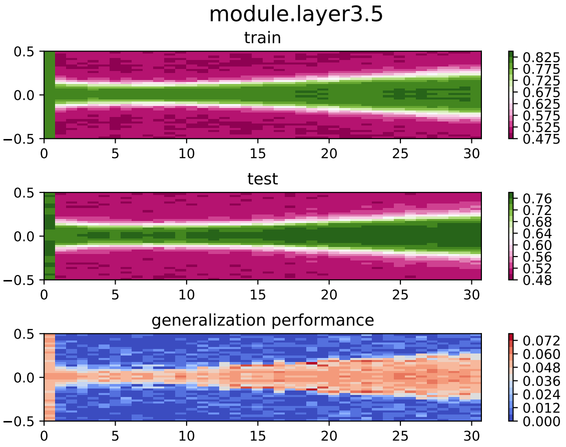


(d) RI-T, optimization path

Figure 10: **Module Criticality Layer3.5**

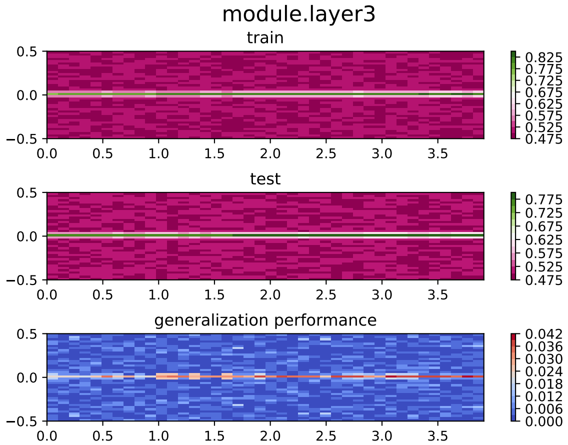


(a) P-T, direct path

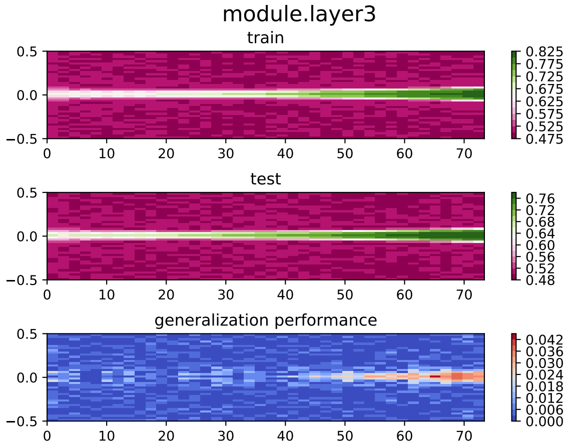


(b) RI-T, direct path

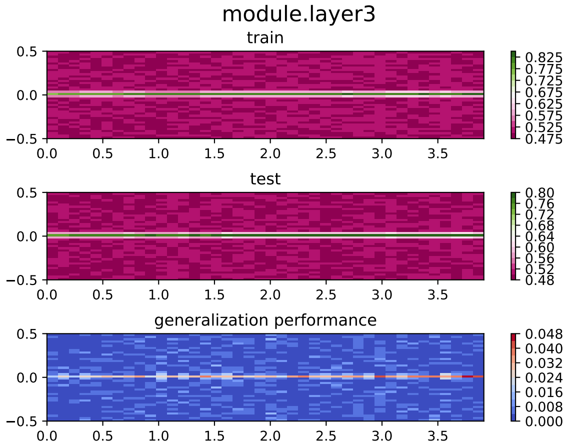


(c) P-T, optimization path

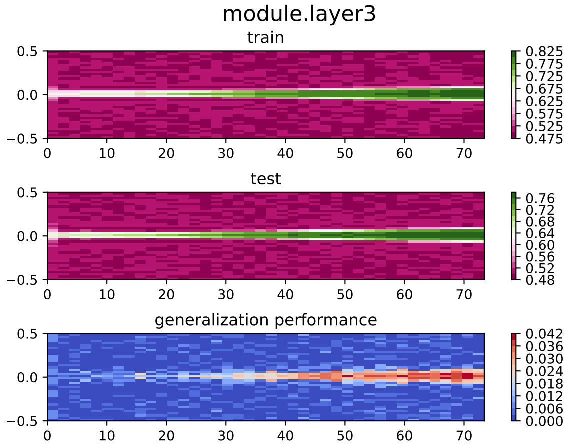


(d) RI-T, optimization path

Figure 11: **Module Criticality Layer3**

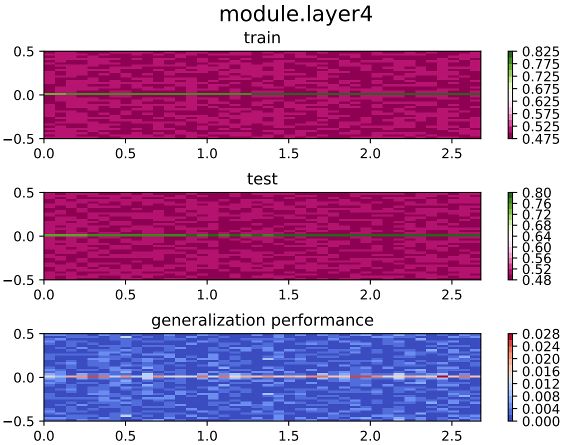


(a) P-T, direct path

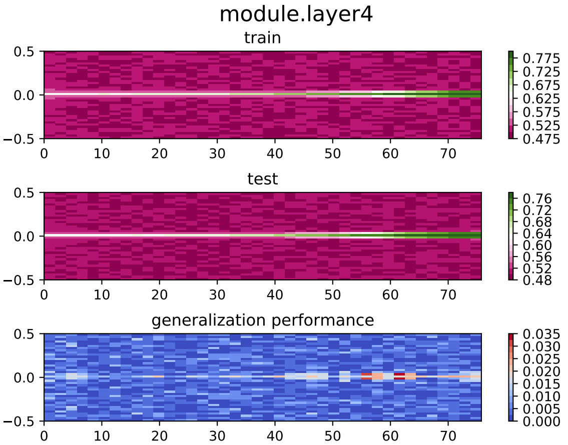


(b) RI-T, direct path

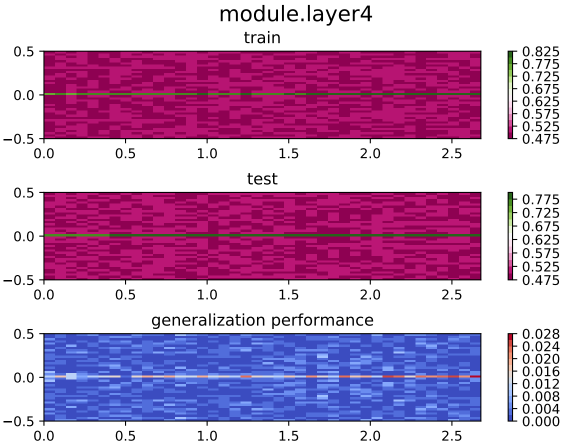


(c) P-T, optimization path

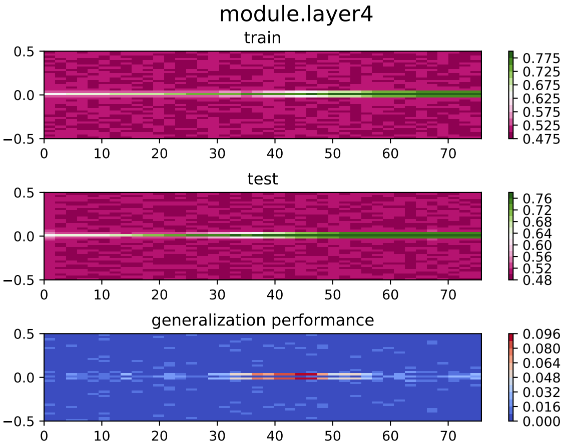


(d) RI-T, optimization path

Figure 12: **Module Criticality Layer4**
