# Supplementary material for: What is being transferred in transfer learning?
Source: arXiv:2008.11687 ancillary file (2021-01-14)
Supplement: Supplementary file 3 [file spectrum_figs_clipart.pdf]

Supplementary Material for  
'What is being transferred in transfer learning?'  
Spectrum plots for Clipart

Behnam Neyshabur\*  
Google  
neyshabur@google.com

Hanie Sedghi\*  
Google Brain  
hsedghi@google.com

Chiyuan Zhang\*  
Google Brain  
chiyuan@google.com

---

\*Equal contribution. Authors ordered randomly.

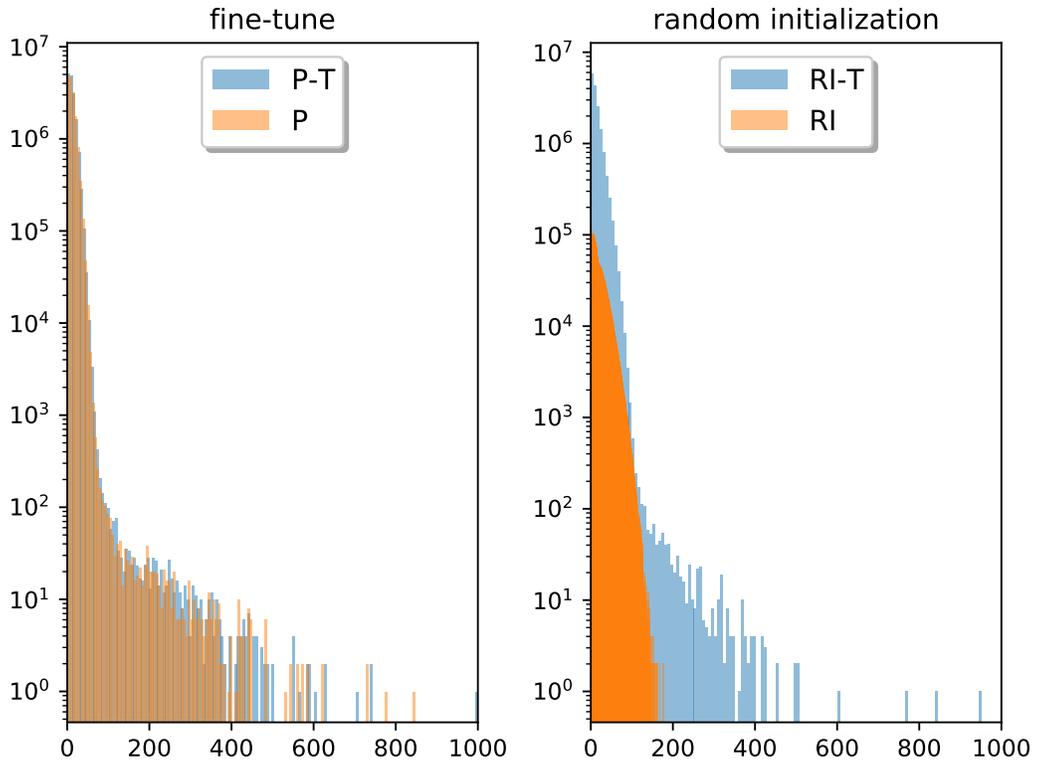

Figure 1: Spectrum for the whole network

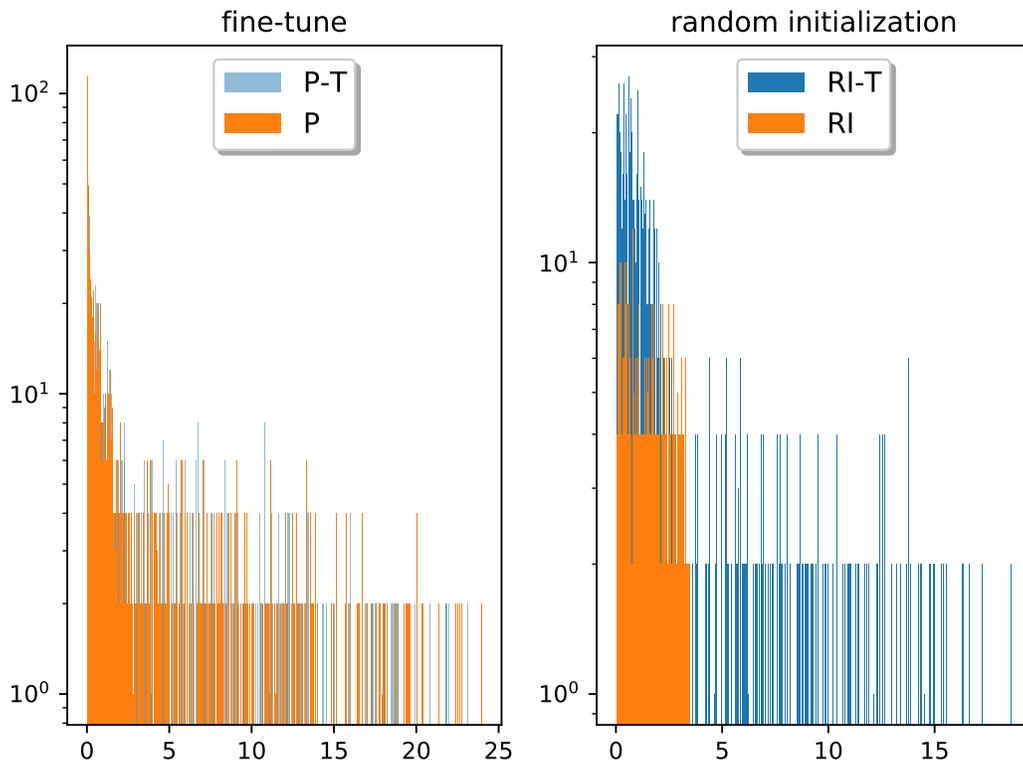

Figure 2: Spectrum Conv1

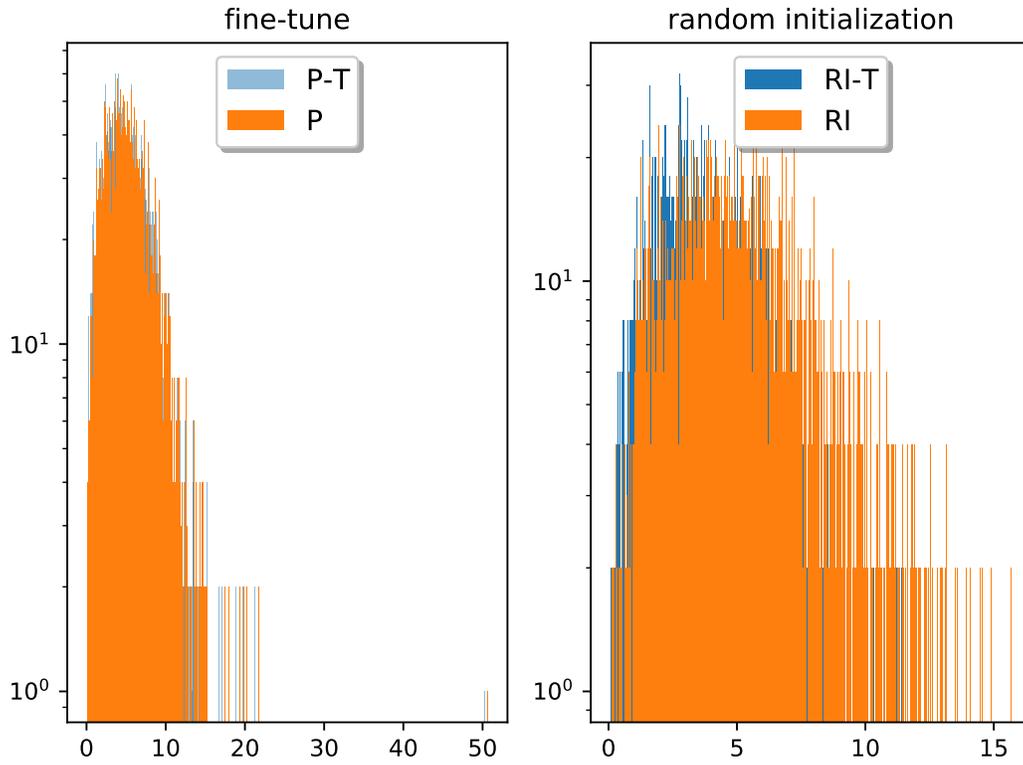

Figure 3: Spectrum Layer1.0 Conv1

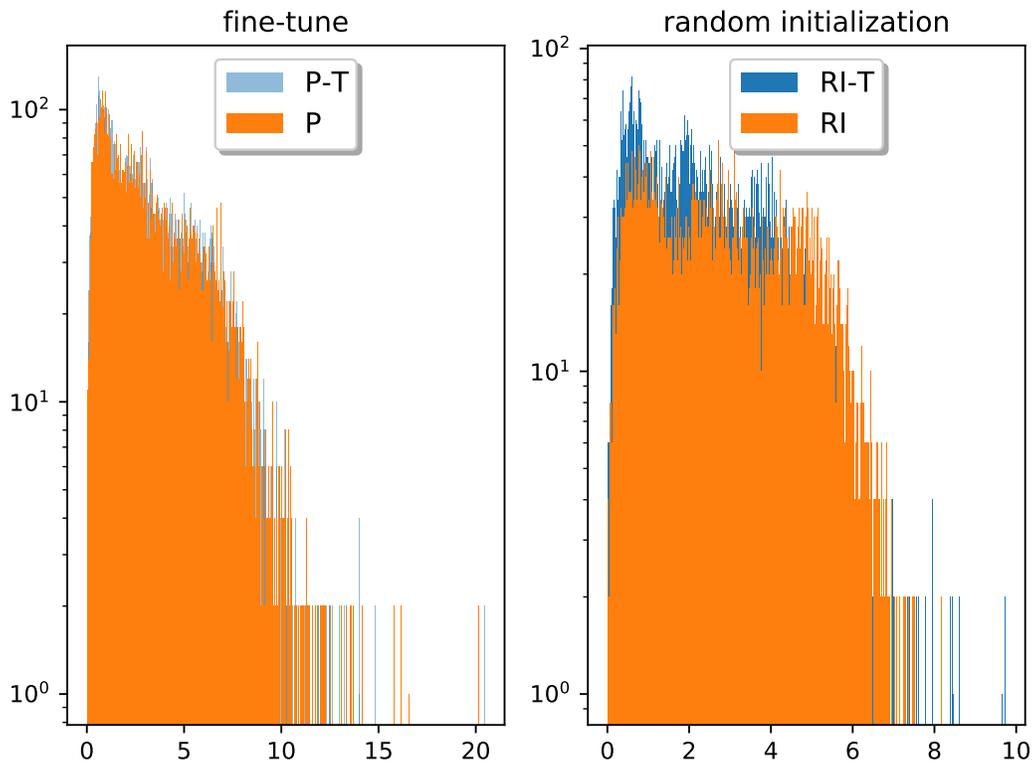

Figure 4: Spectrum Layer1.0 Conv2

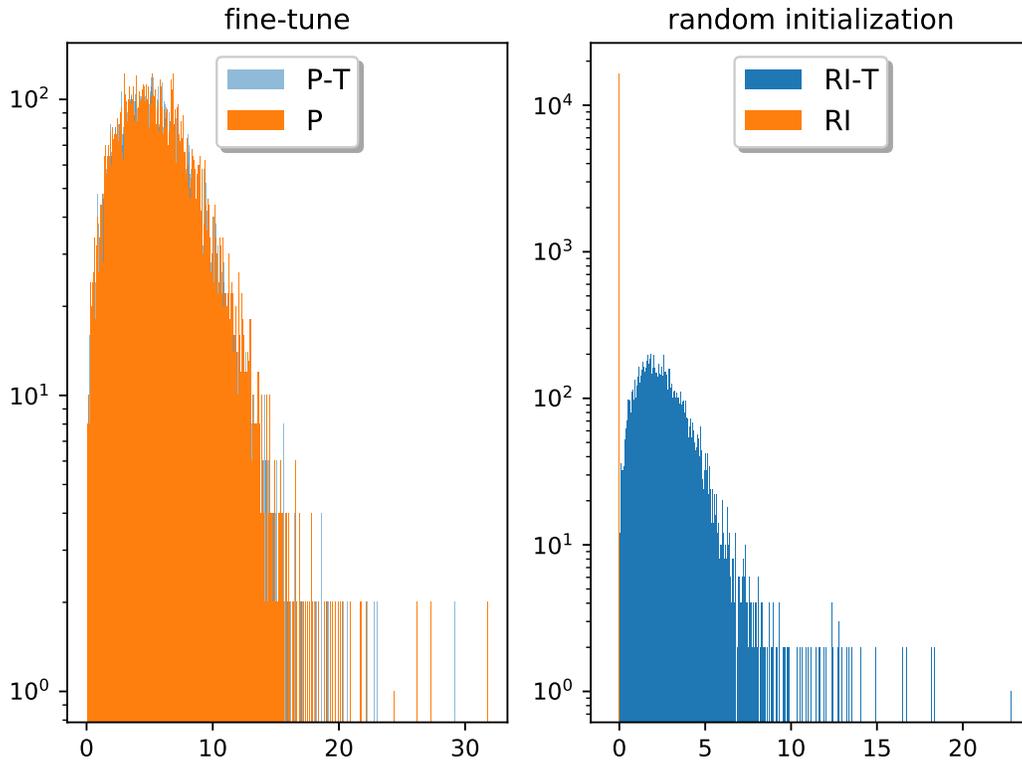

Figure 5: Spectrum Layer1.0 Conv3

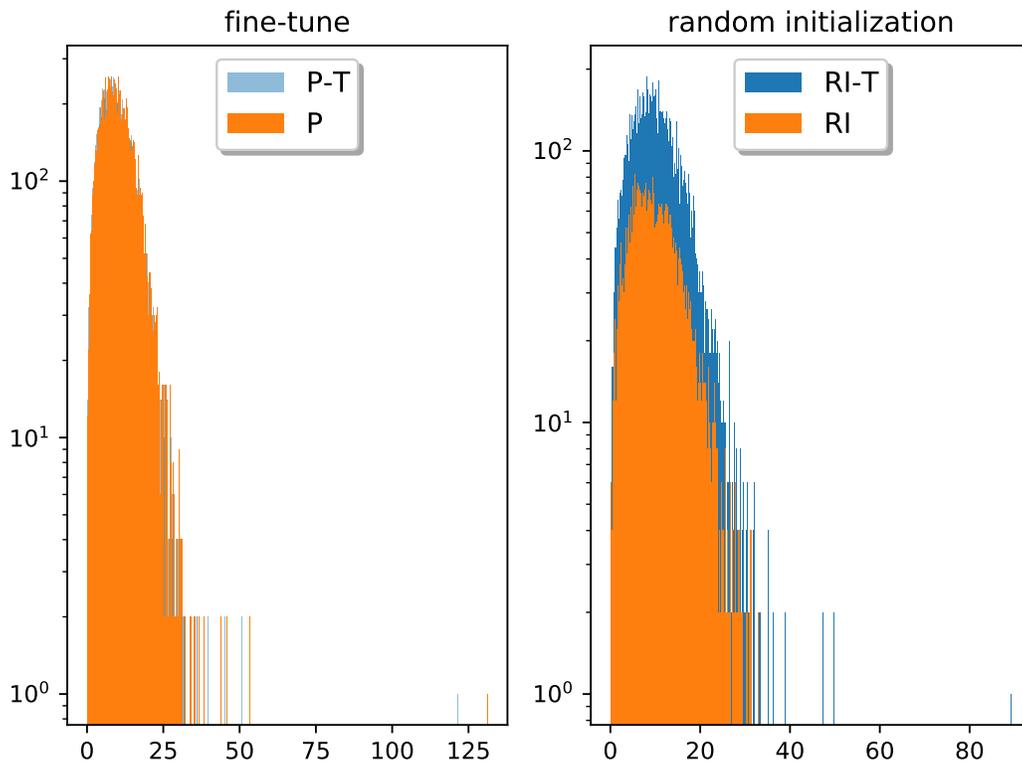

Figure 6: Spectrum Layer1.0 Downsample

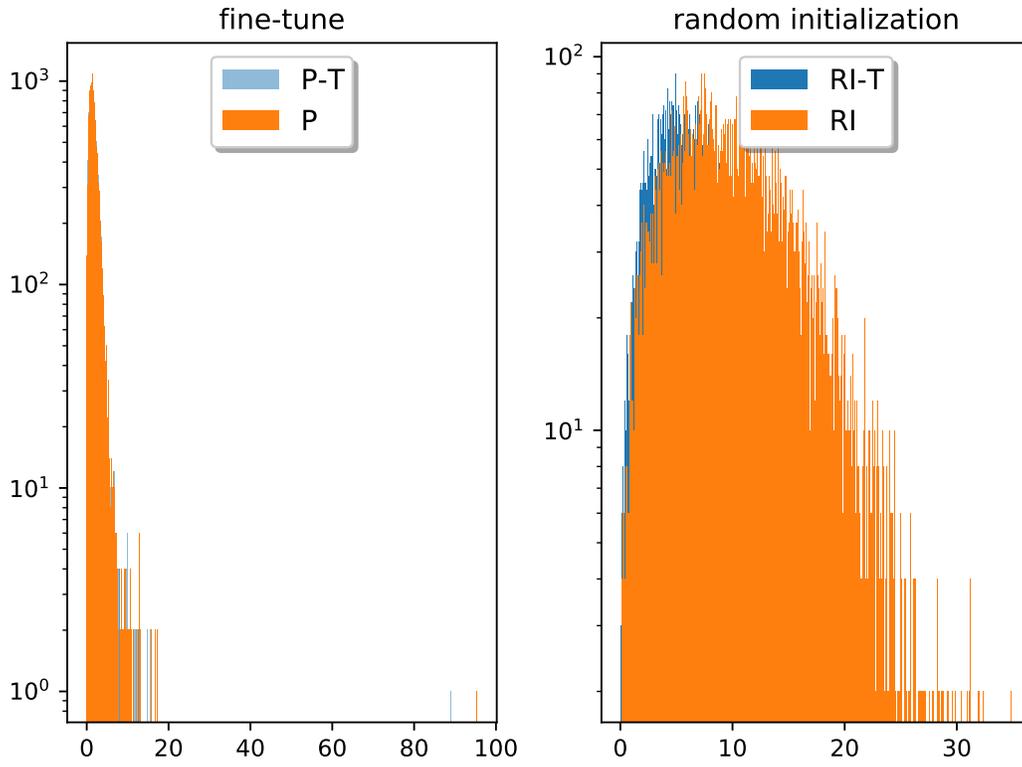

Figure 7: Spectrum Layer1.1 Conv1

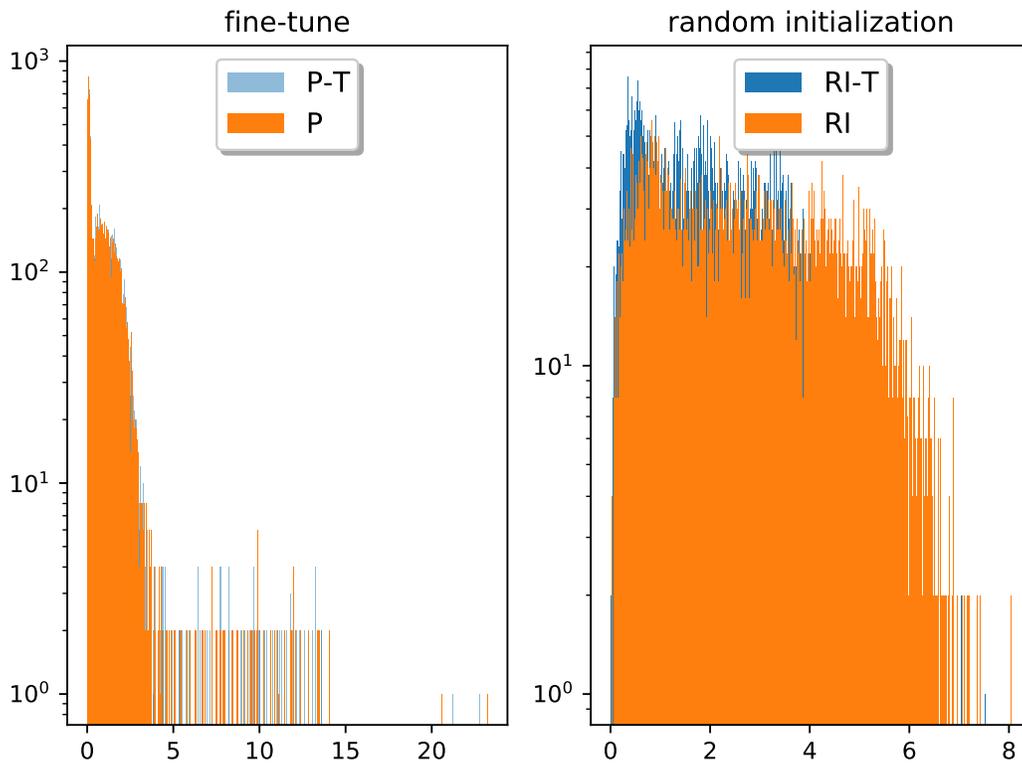

Figure 8: Spectrum Layer1.1 Conv2

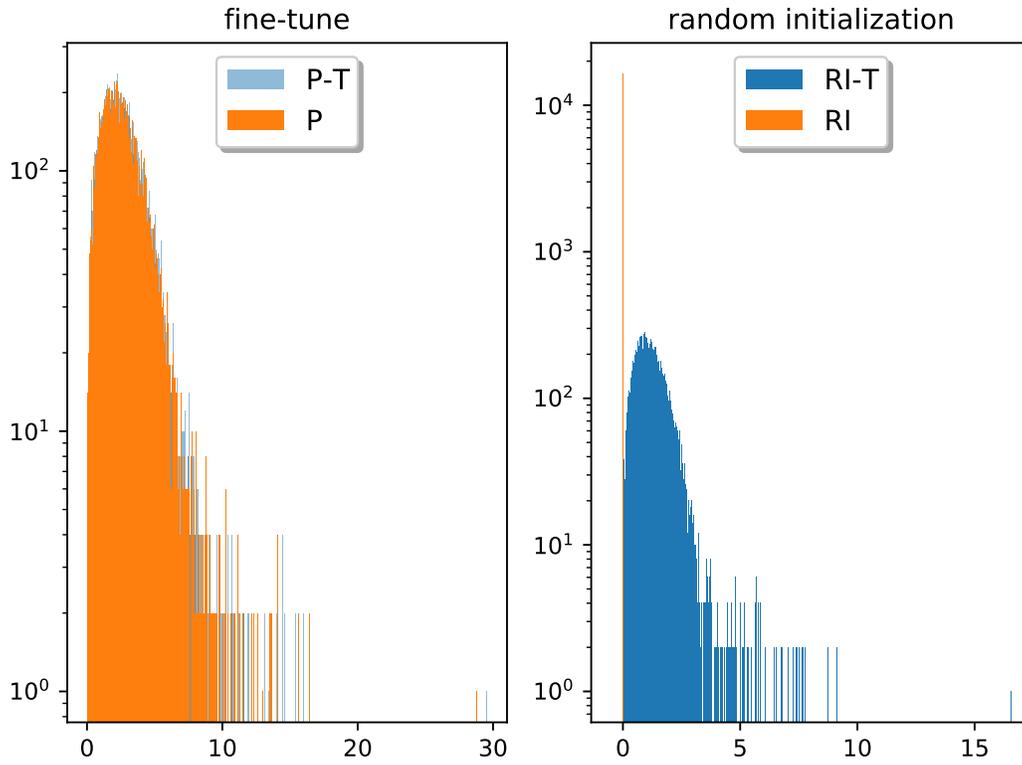

Figure 9: Spectrum Layer1.1 Conv3

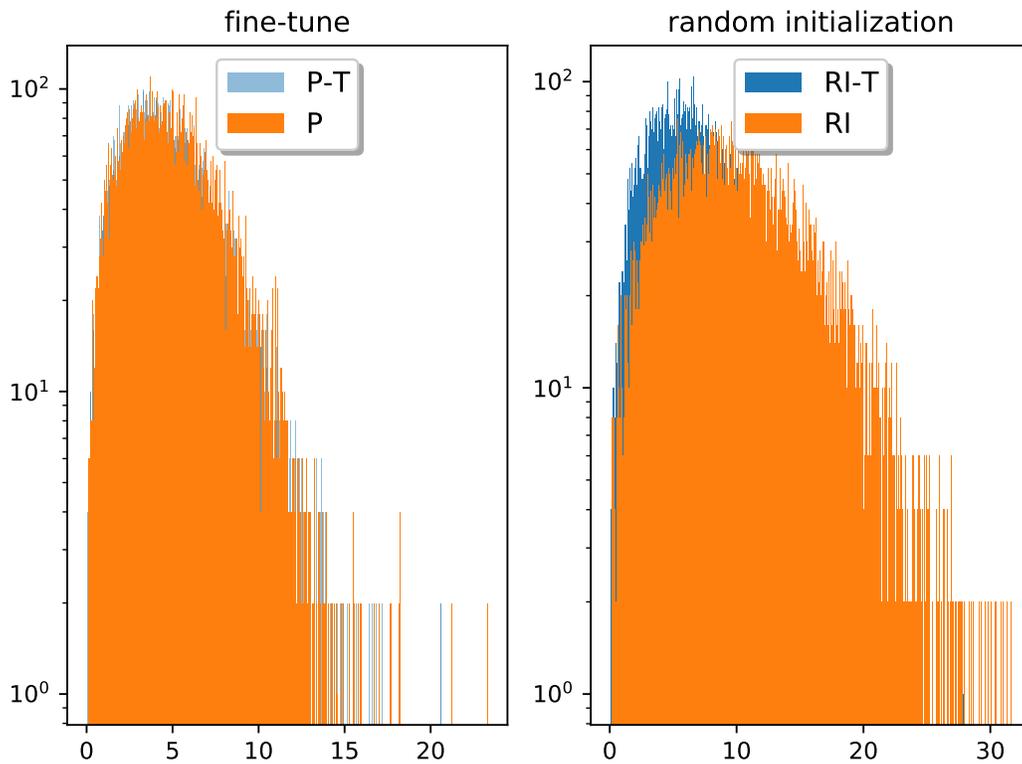

Figure 10: Spectrum Layer1.2 Conv1

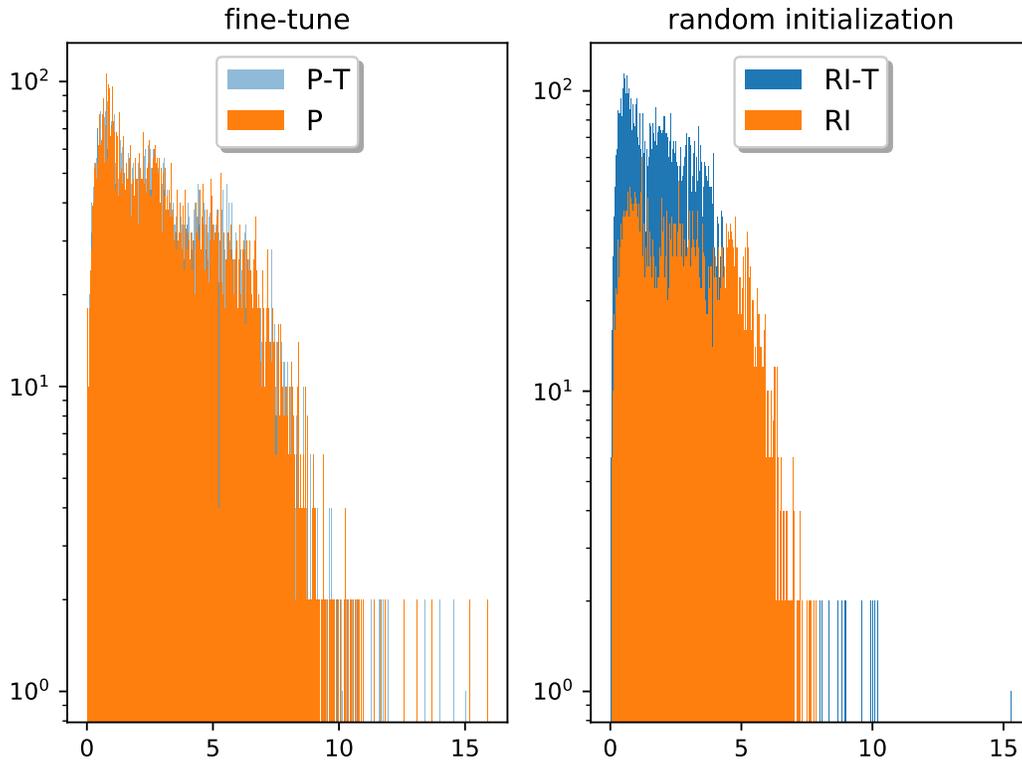

Figure 11: Spectrum Layer1.2 Conv2

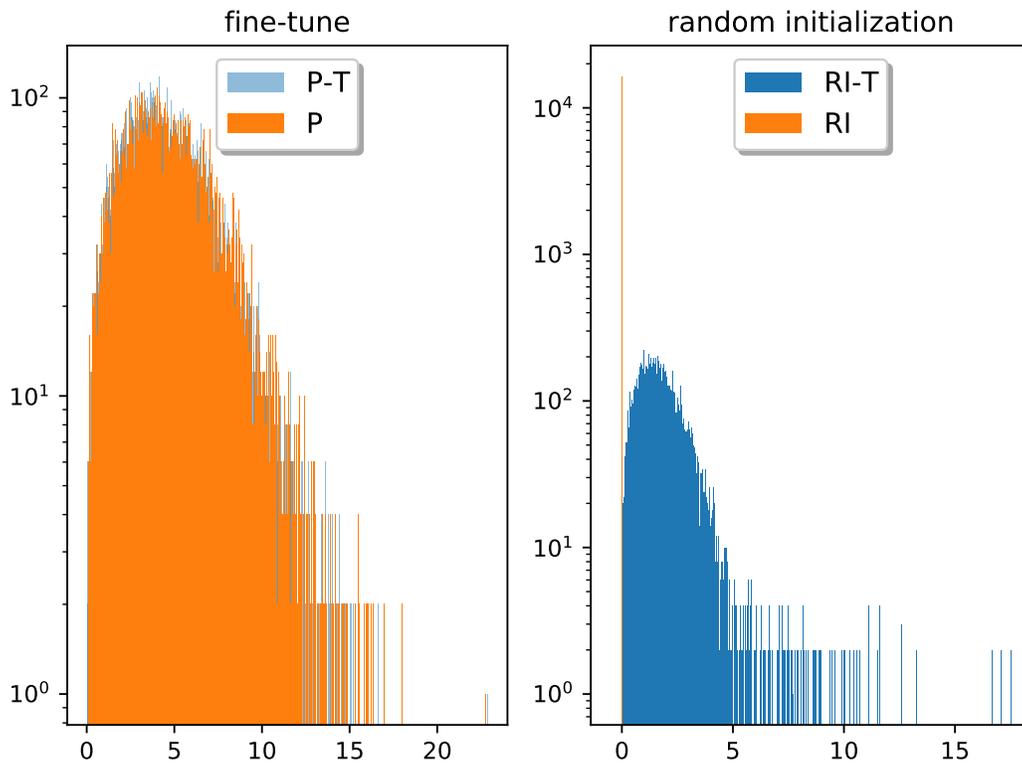

Figure 12: Spectrum Layer1.2 Conv3

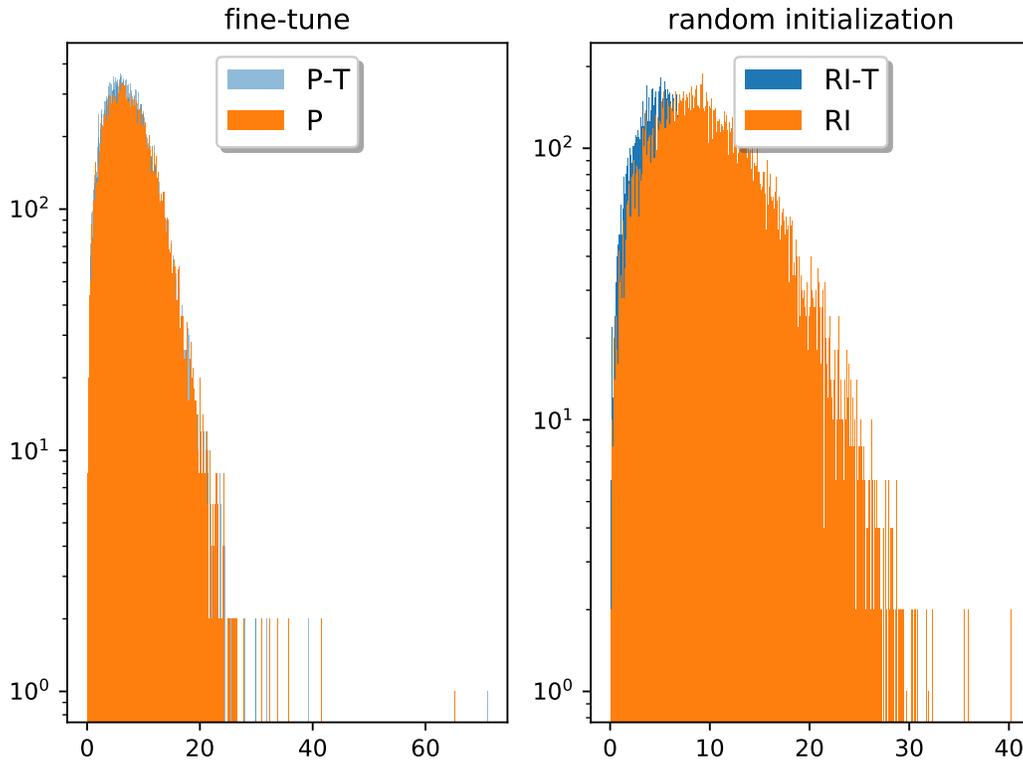

Figure 13: Spectrum Layer2.0 Conv1

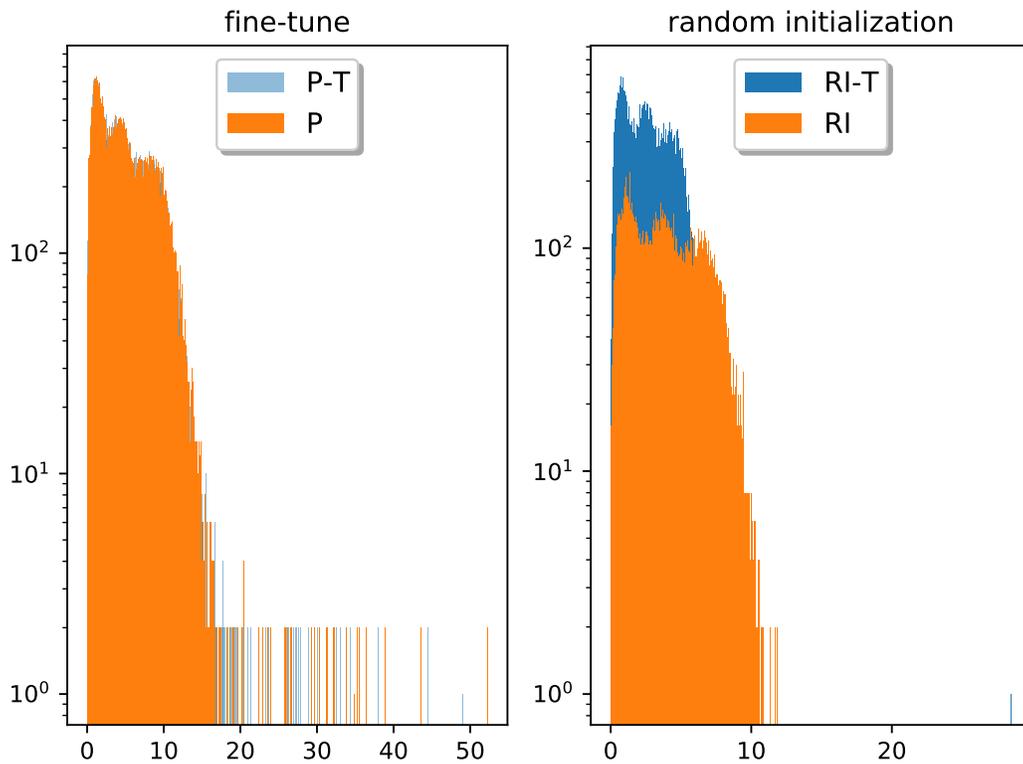

Figure 14: Spectrum Layer2.0 Conv2

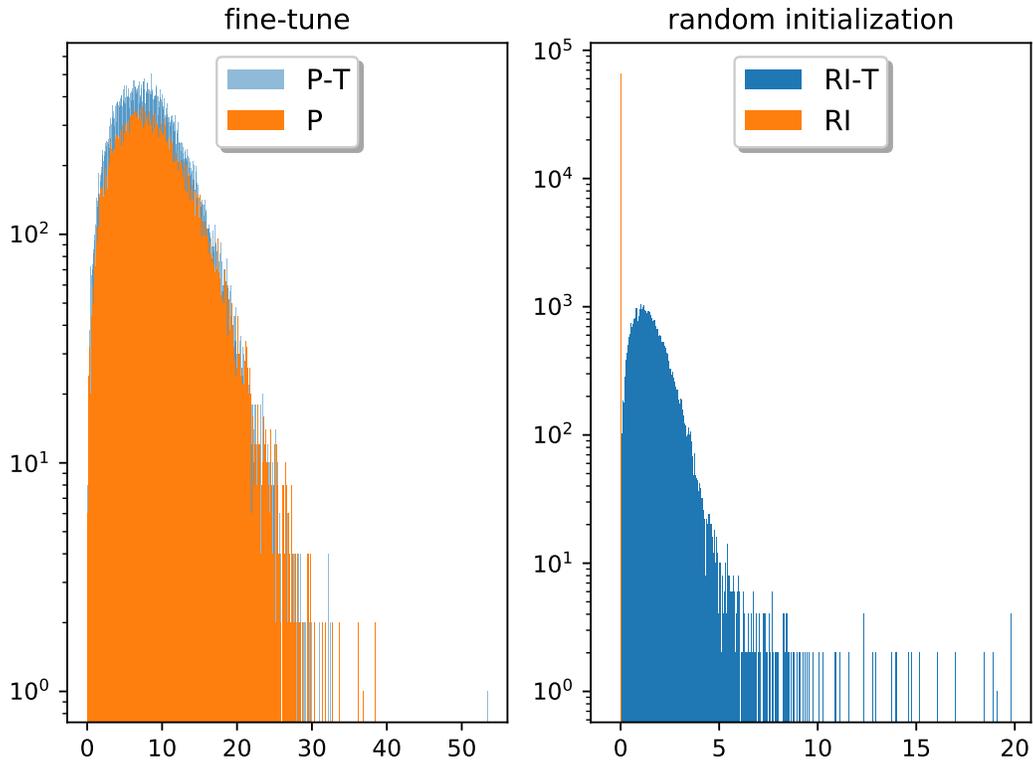

Figure 15: Spectrum Layer2.0 Conv3

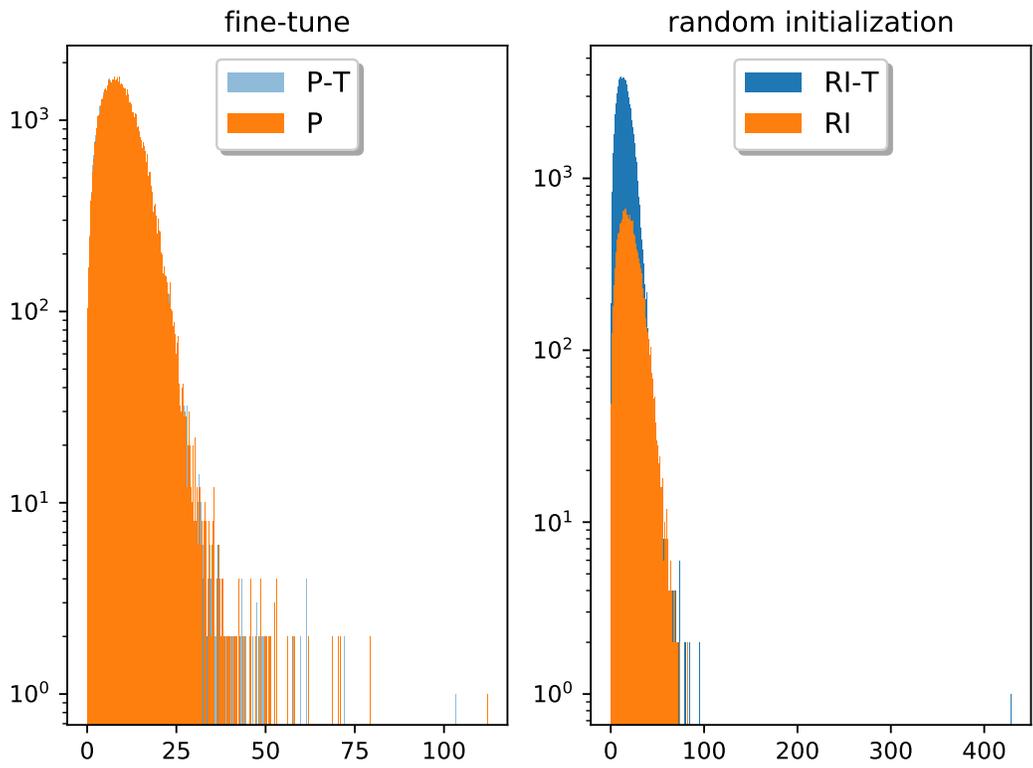

Figure 16: Spectrum Layer2.0 Downsample

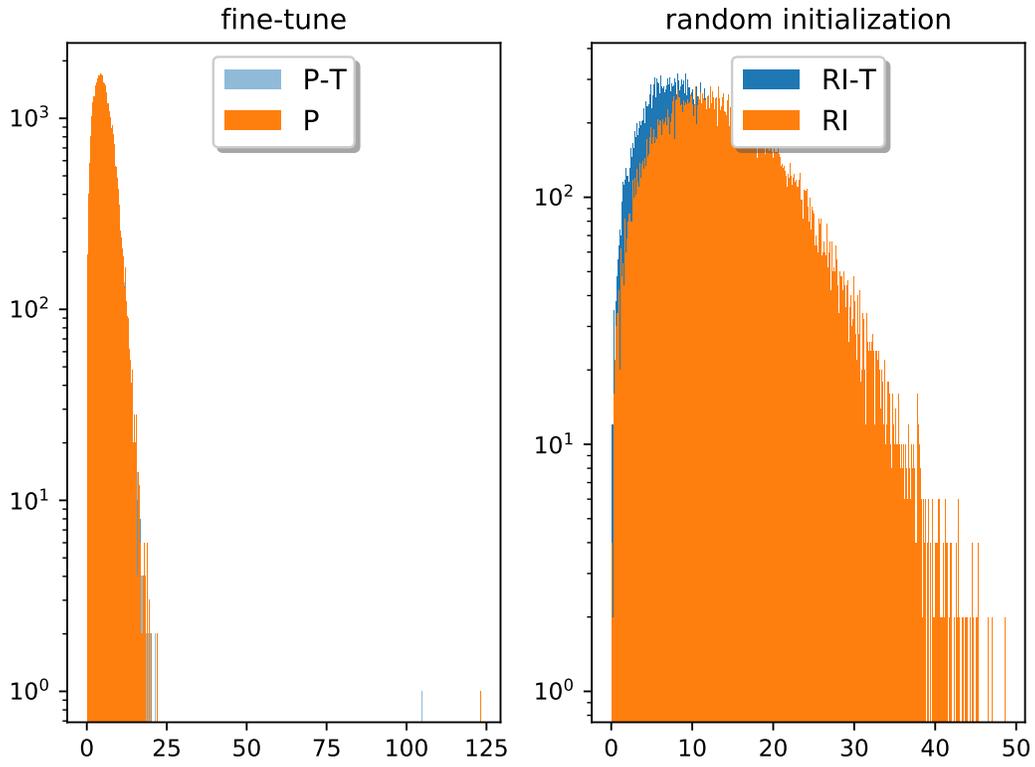

Figure 17: Spectrum Layer2.1 Conv1

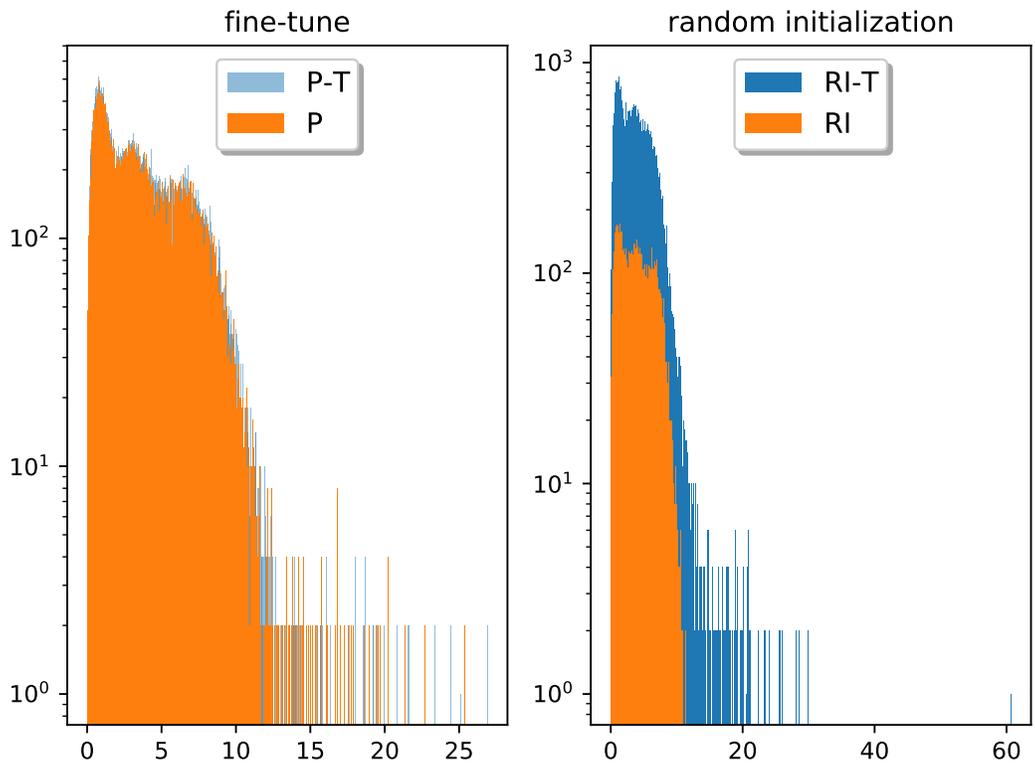

Figure 18: Spectrum Layer2.1 Conv2

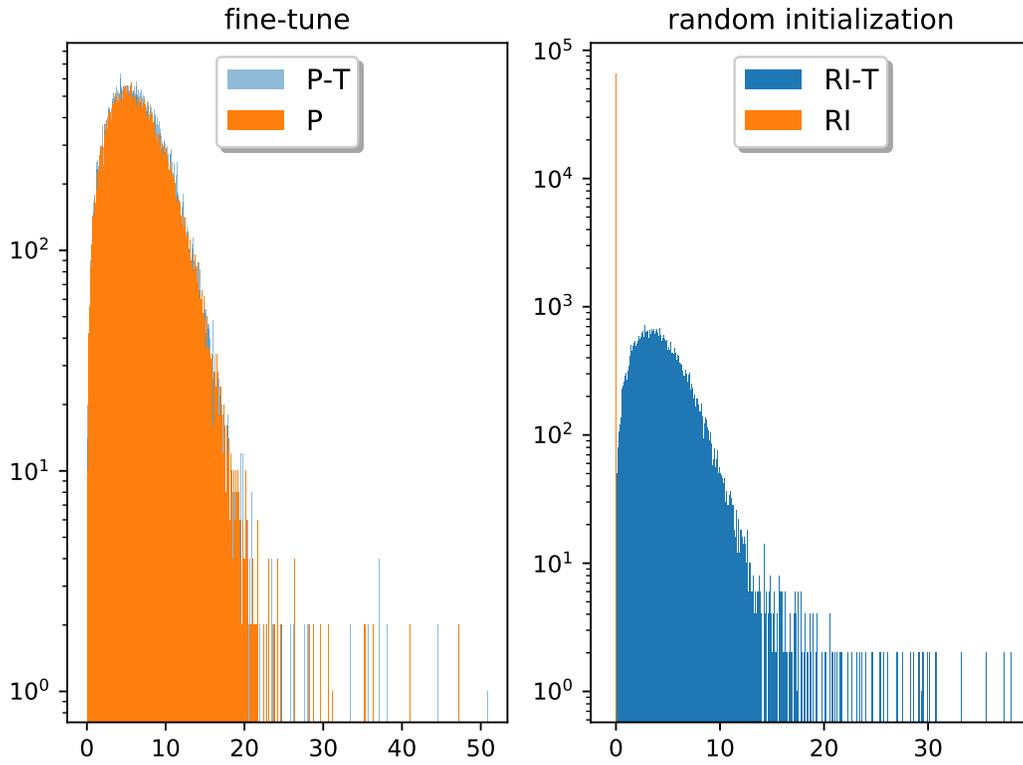

Figure 19: Spectrum Layer2.1 Conv3

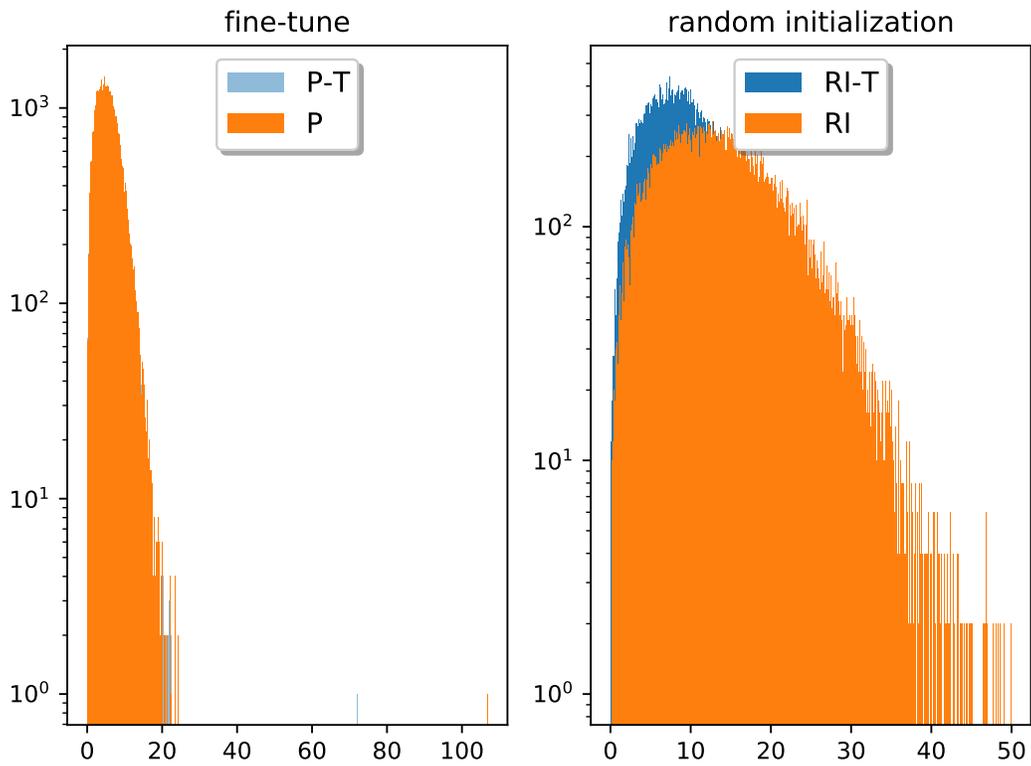

Figure 20: Spectrum Layer2.2 Conv1

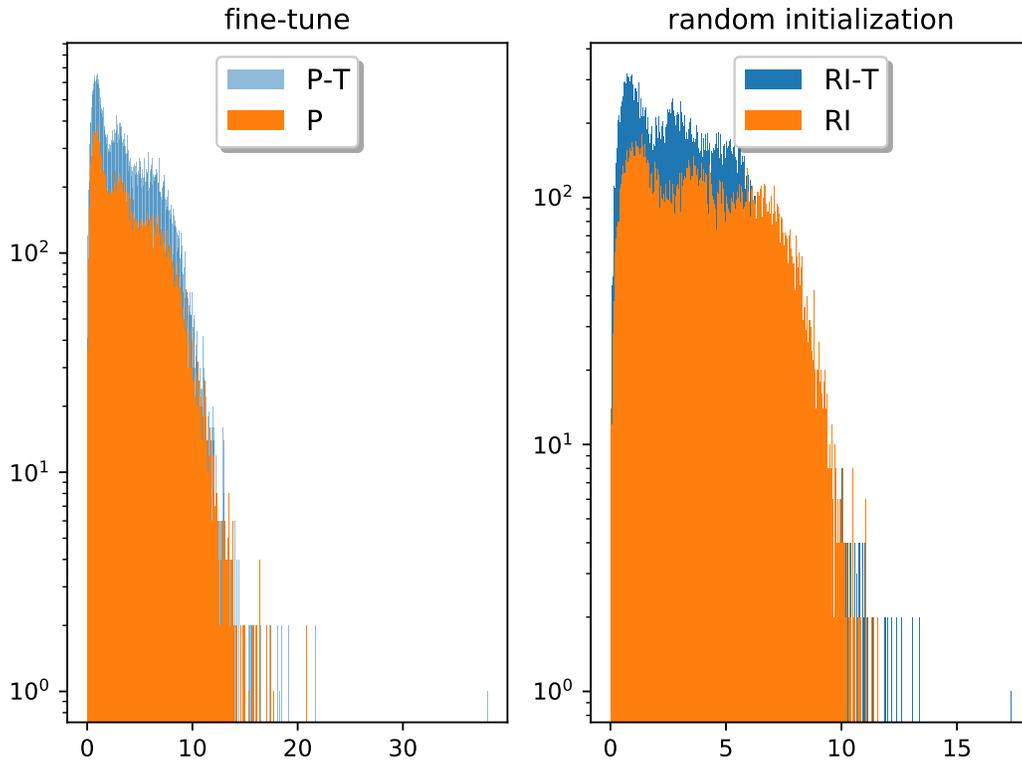

Figure 21: Spectrum Layer2.2 Conv2

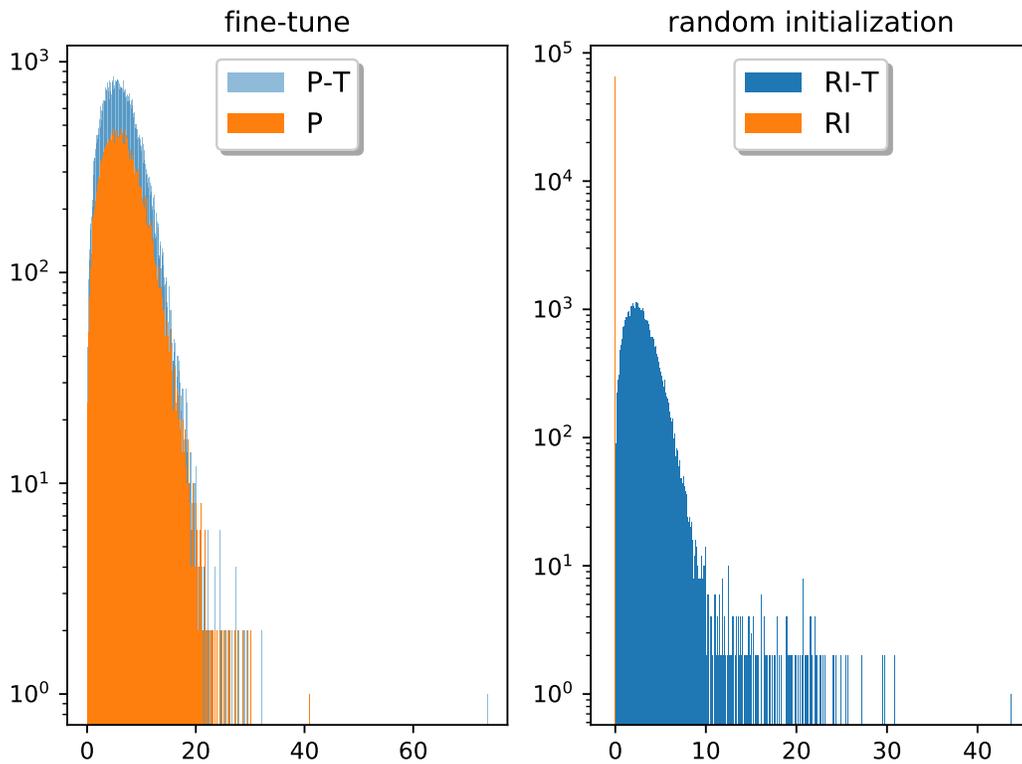

Figure 22: Spectrum Layer2.2 Conv3

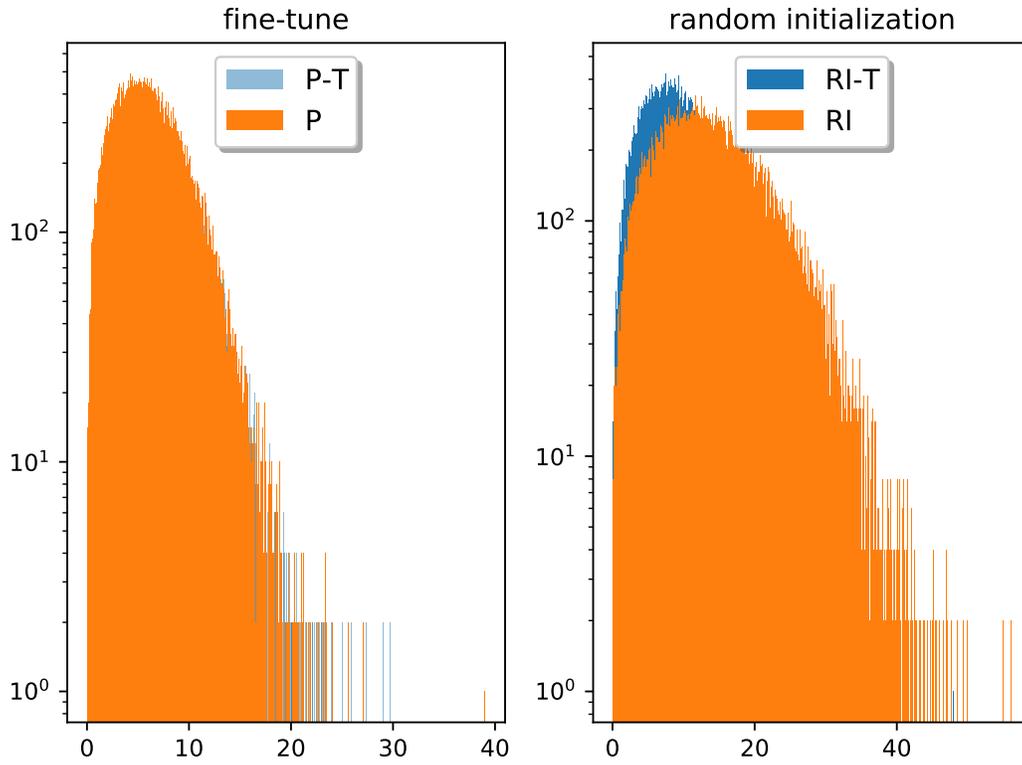

Figure 23: Spectrum Layer2.3 Conv1

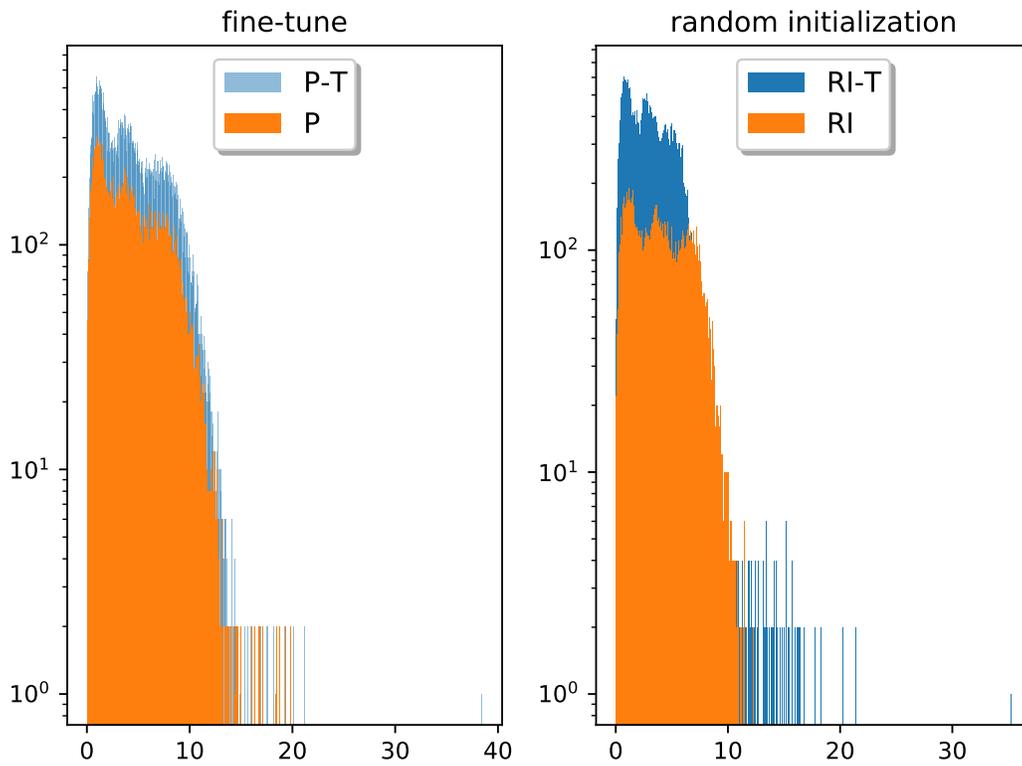

Figure 24: Spectrum Layer2.3 Conv2

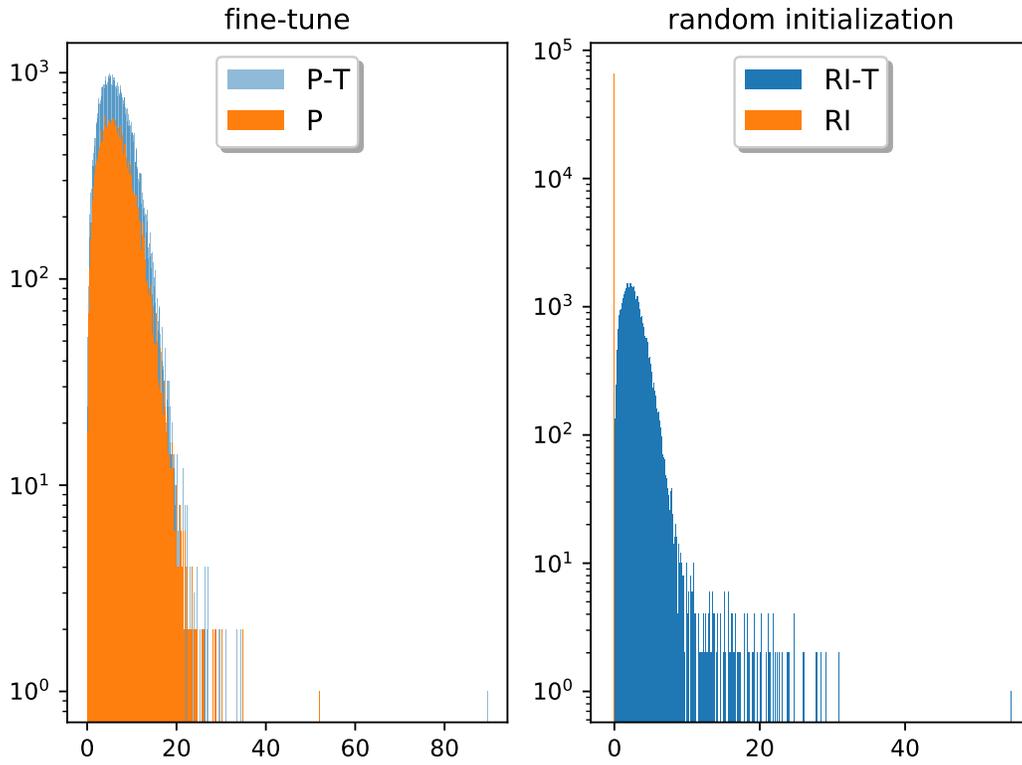

Figure 25: Spectrum Layer2.3 Conv3

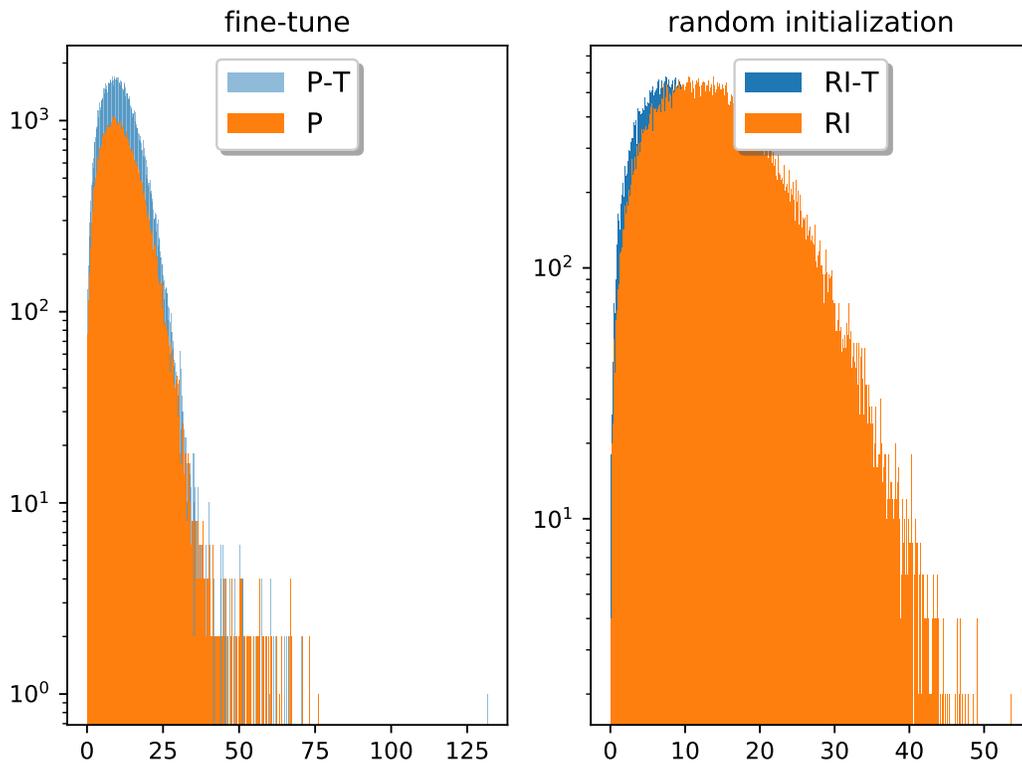

Figure 26: Spectrum Layer3.0 Conv1

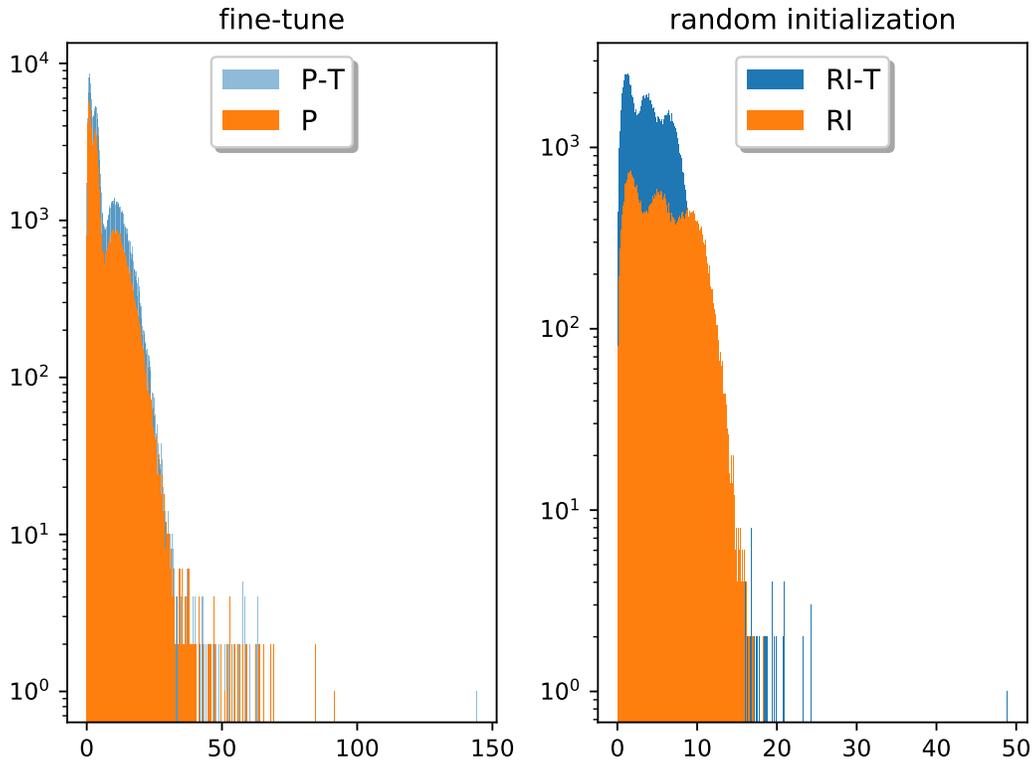

Figure 27: Spectrum Layer3.0 Conv2

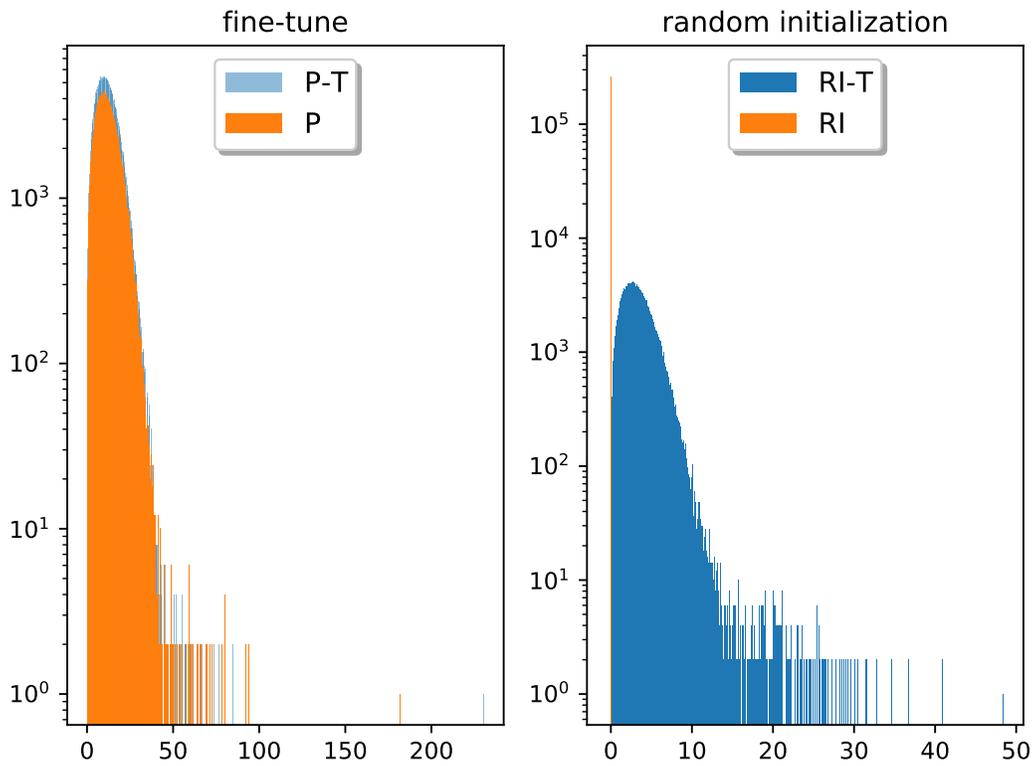

Figure 28: Spectrum Layer3.0 Conv3

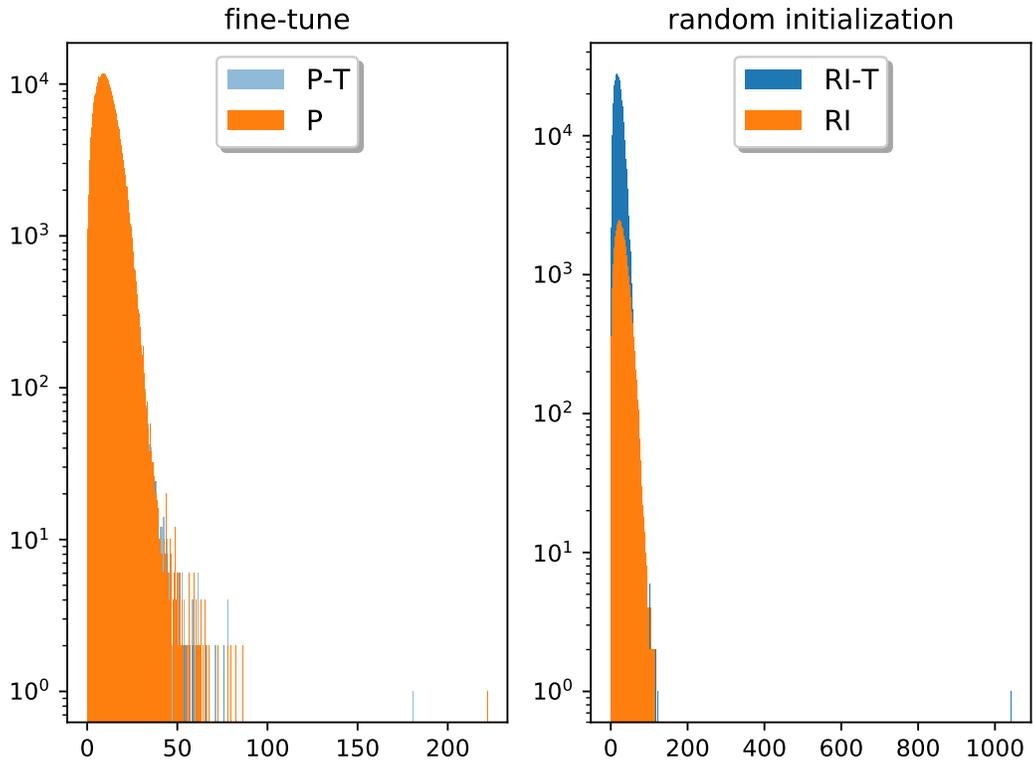

Figure 29: Spectrum Layer3.0 Downsample

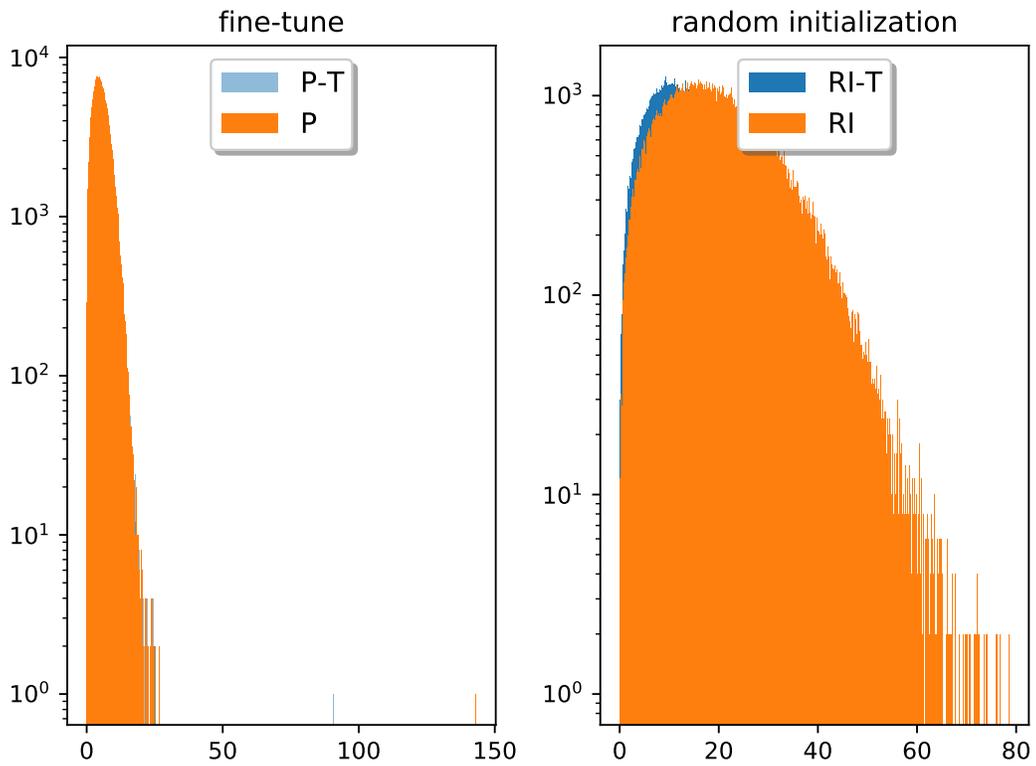

Figure 30: Spectrum Layer3.1 Conv1

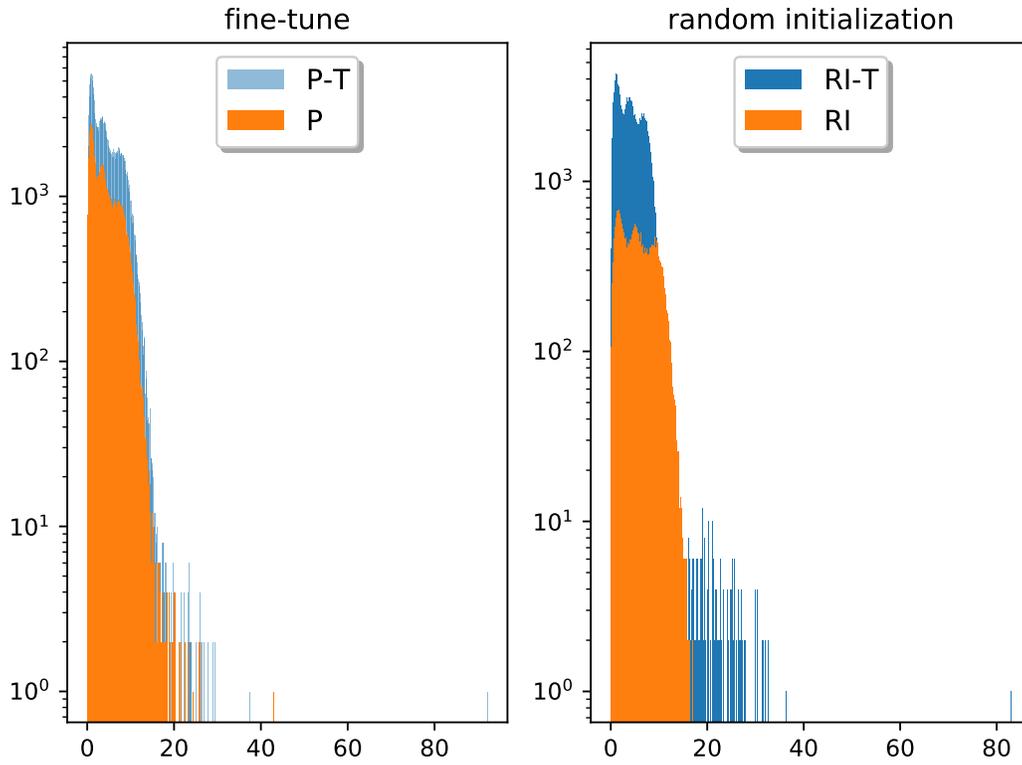

Figure 31: Spectrum Layer3.1 Conv2

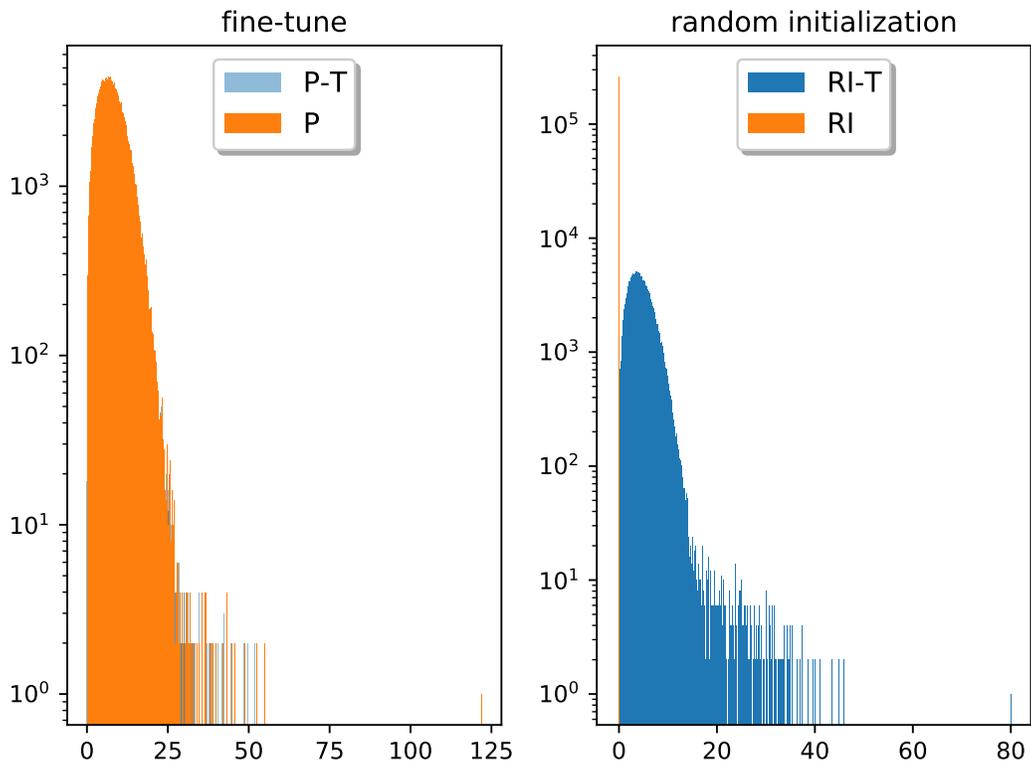

Figure 32: Spectrum Layer3.1 Conv3

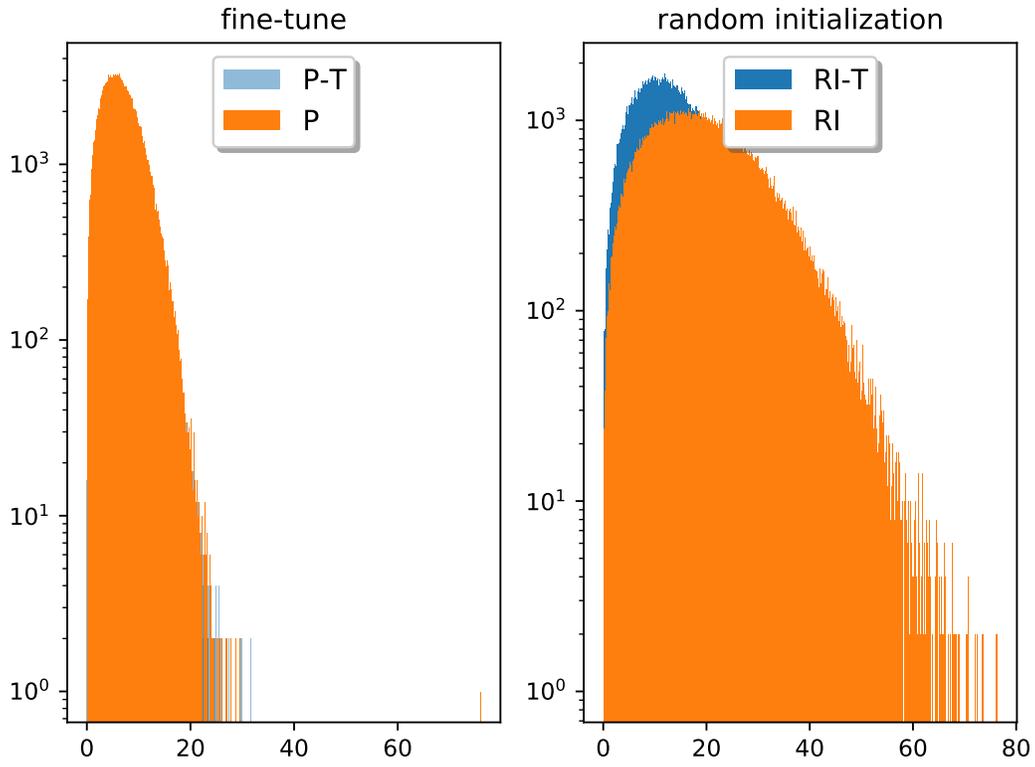

Figure 33: Spectrum Layer3.2 Conv1

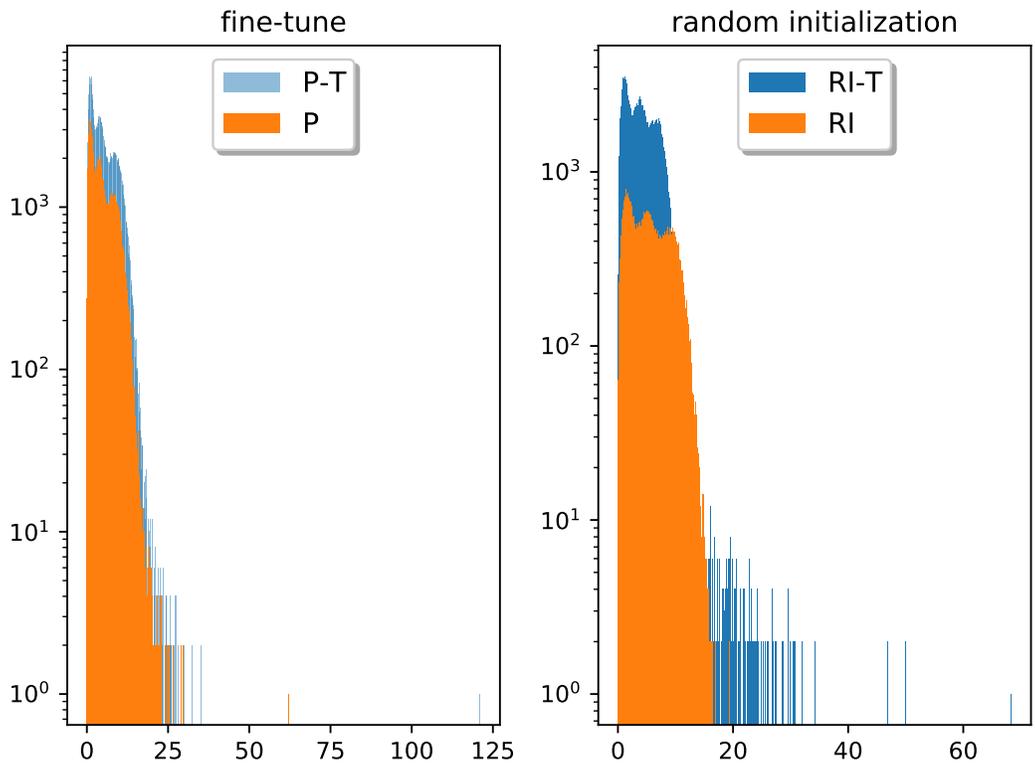

Figure 34: Spectrum Layer3.2 Conv2

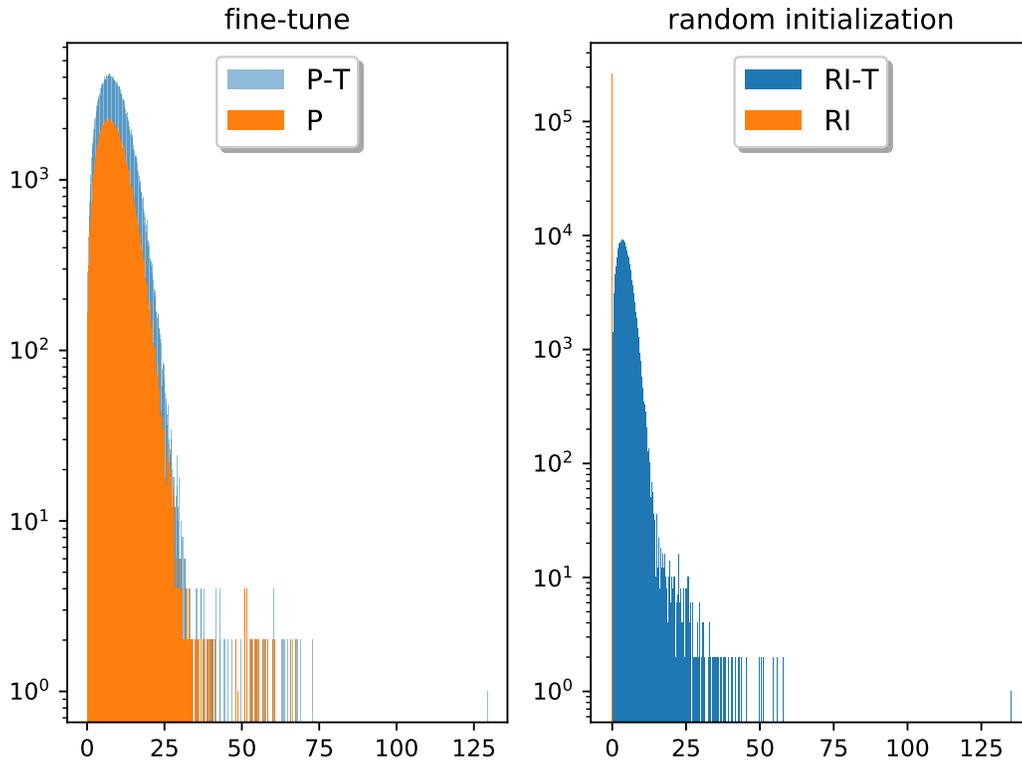

Figure 35: Spectrum Layer3.2 Conv3

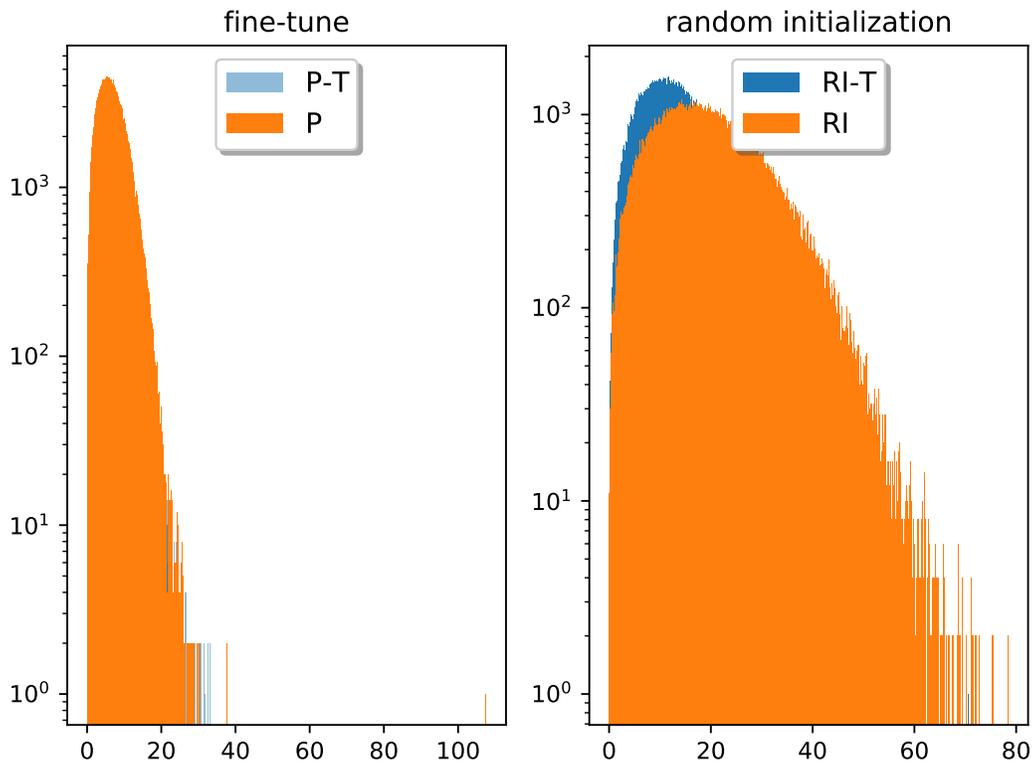

Figure 36: Spectrum Layer3.3 Conv1

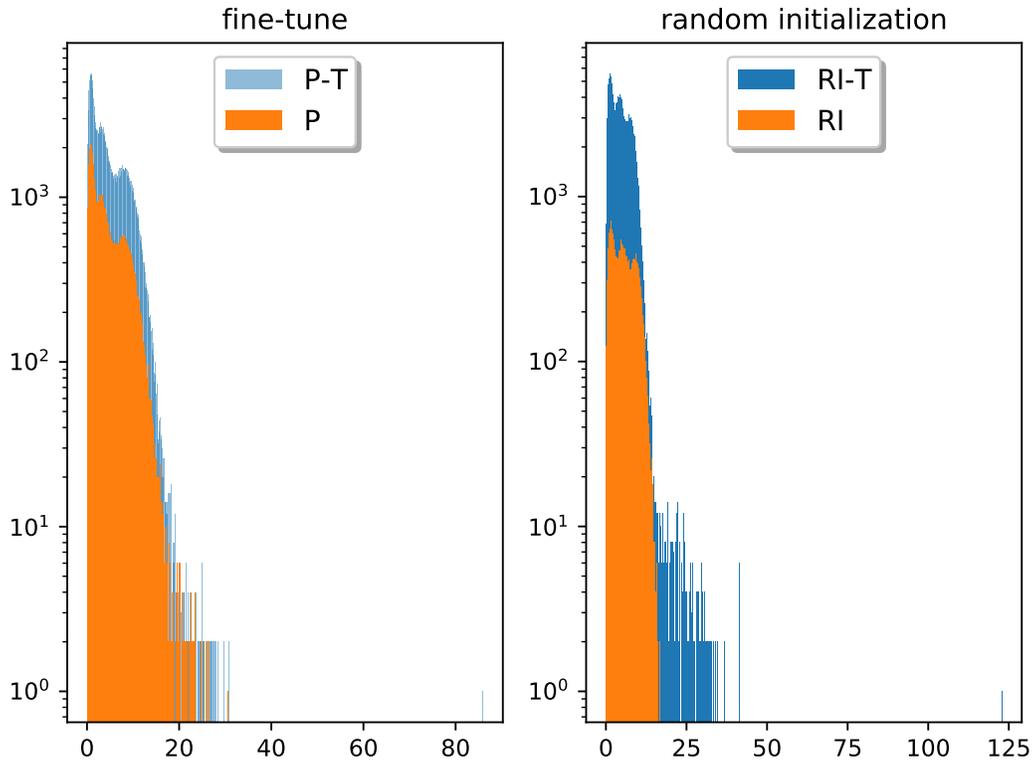

Figure 37: Spectrum Layer3.3 Conv2

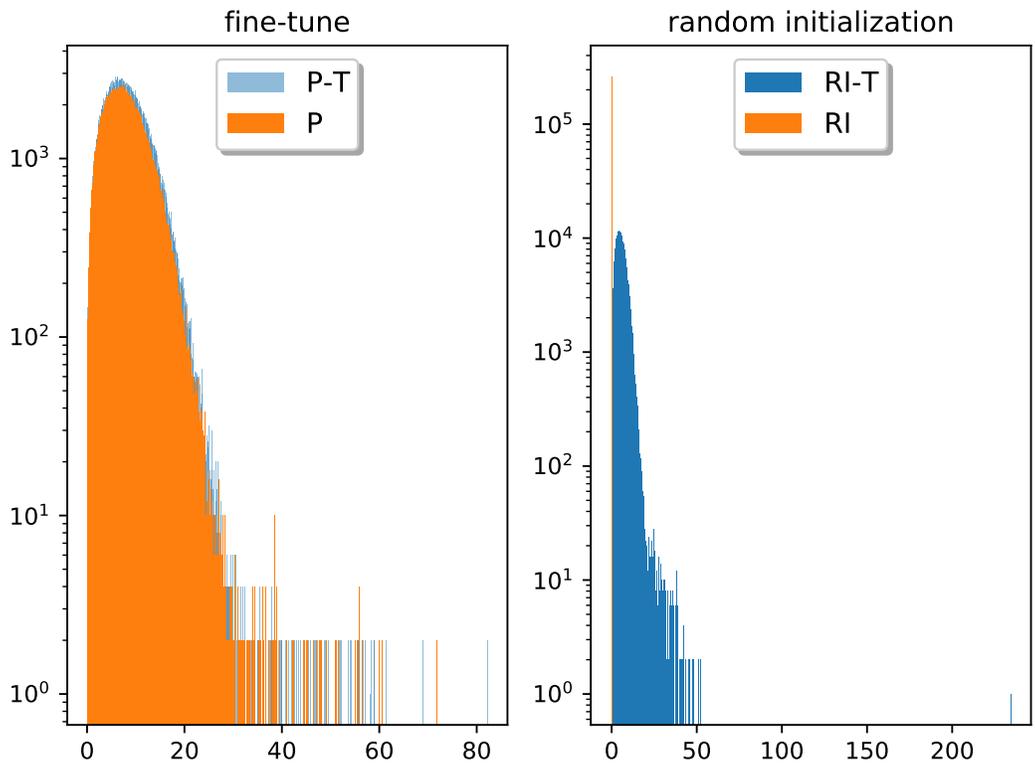

Figure 38: Spectrum Layer3.3 Conv3

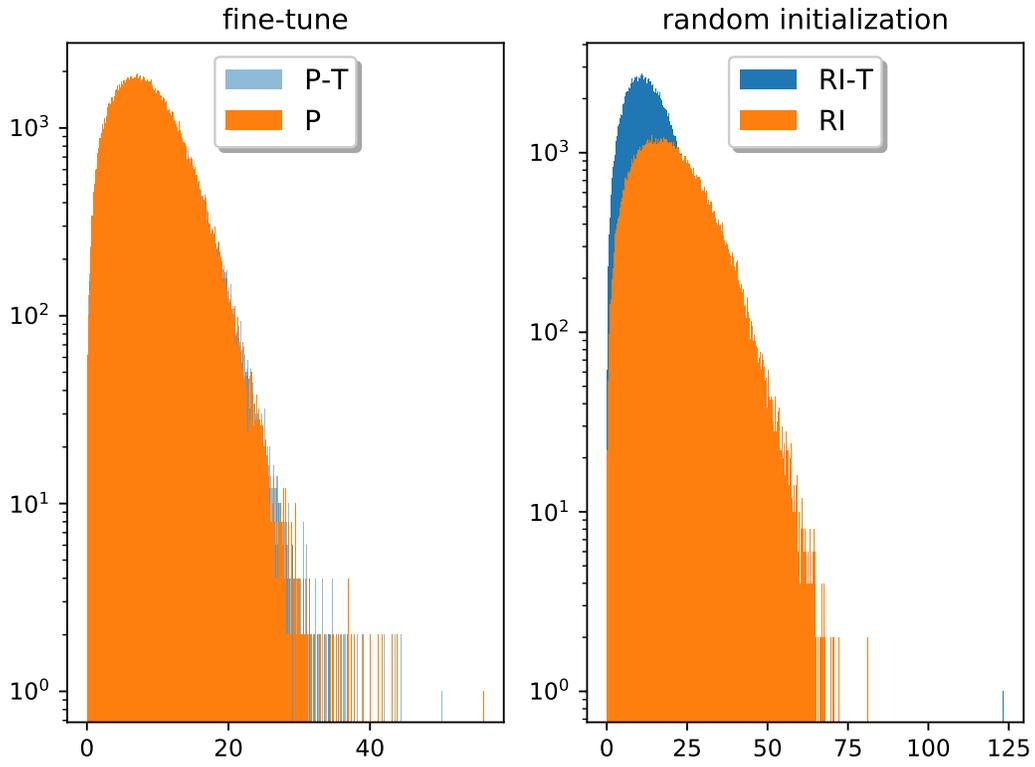

Figure 39: Spectrum Layer3.4 Conv1

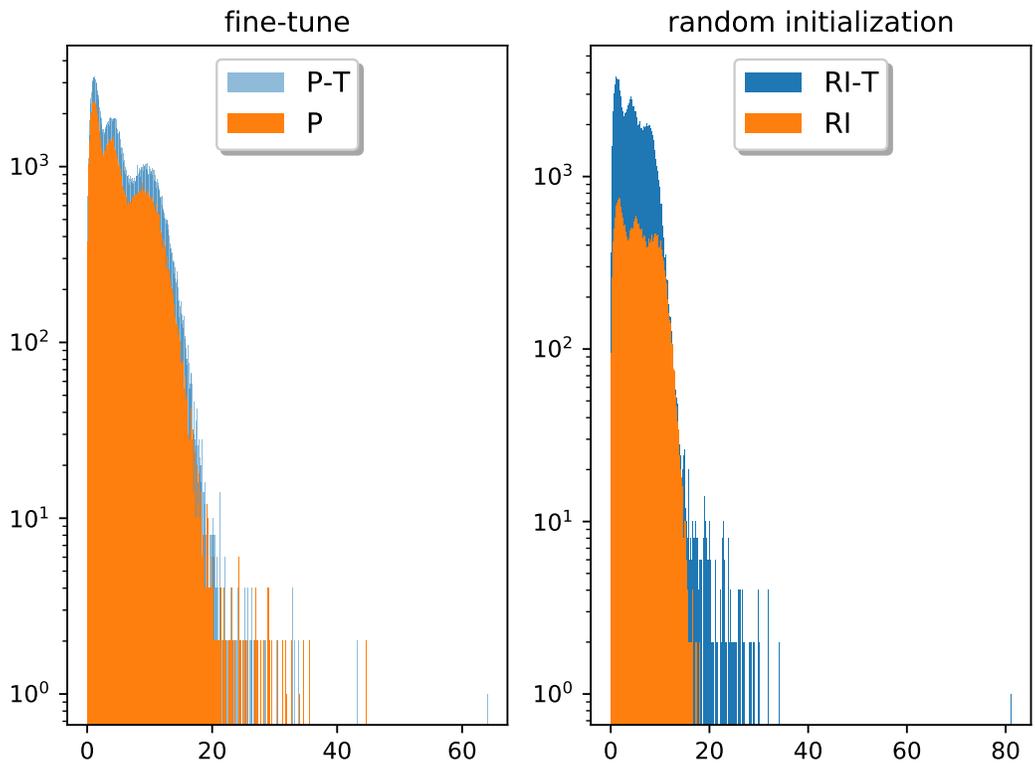

Figure 40: Spectrum Layer3.4 Conv2

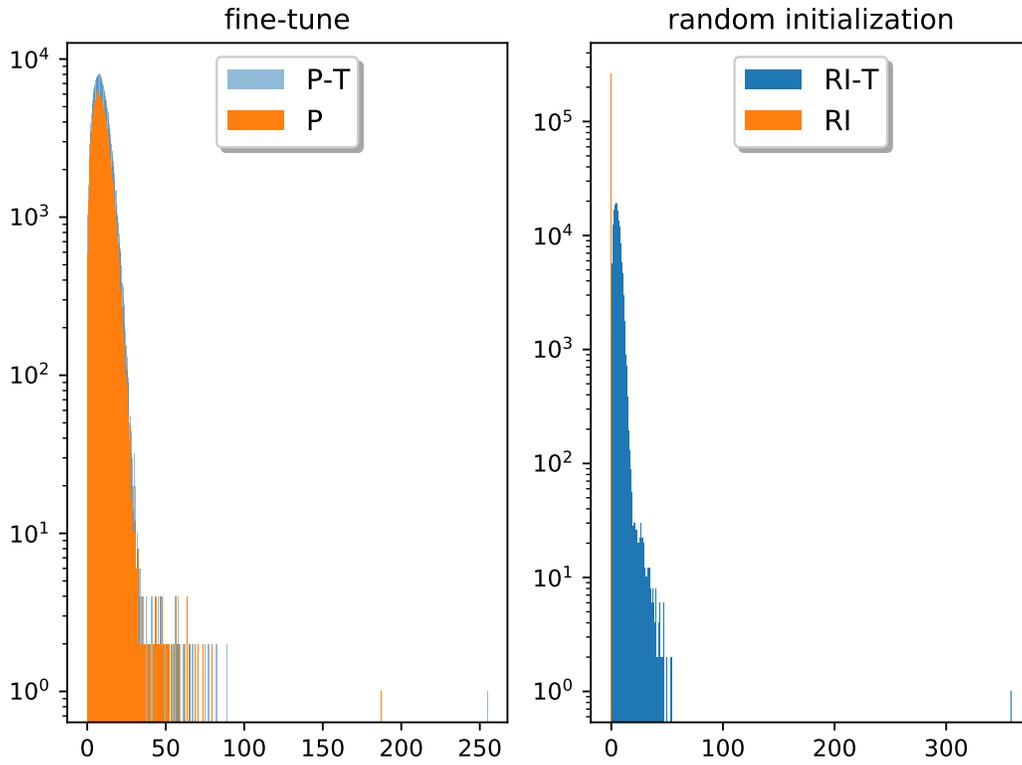

Figure 41: Spectrum Layer3.4 Conv3

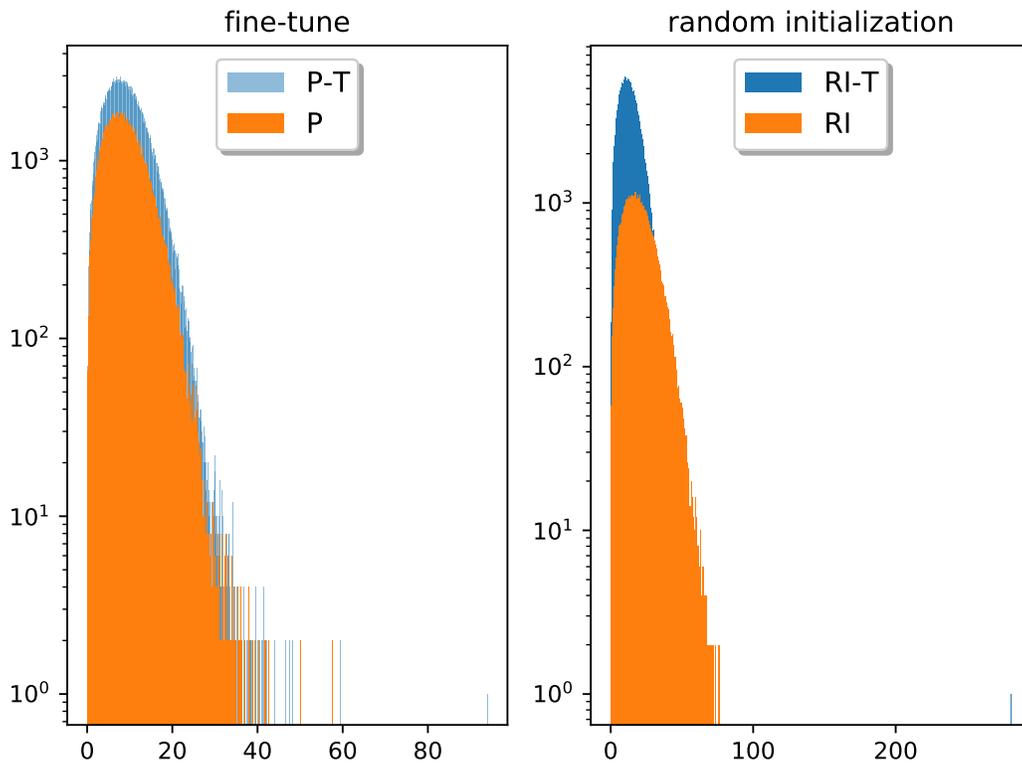

Figure 42: Spectrum Layer3.5 Conv1

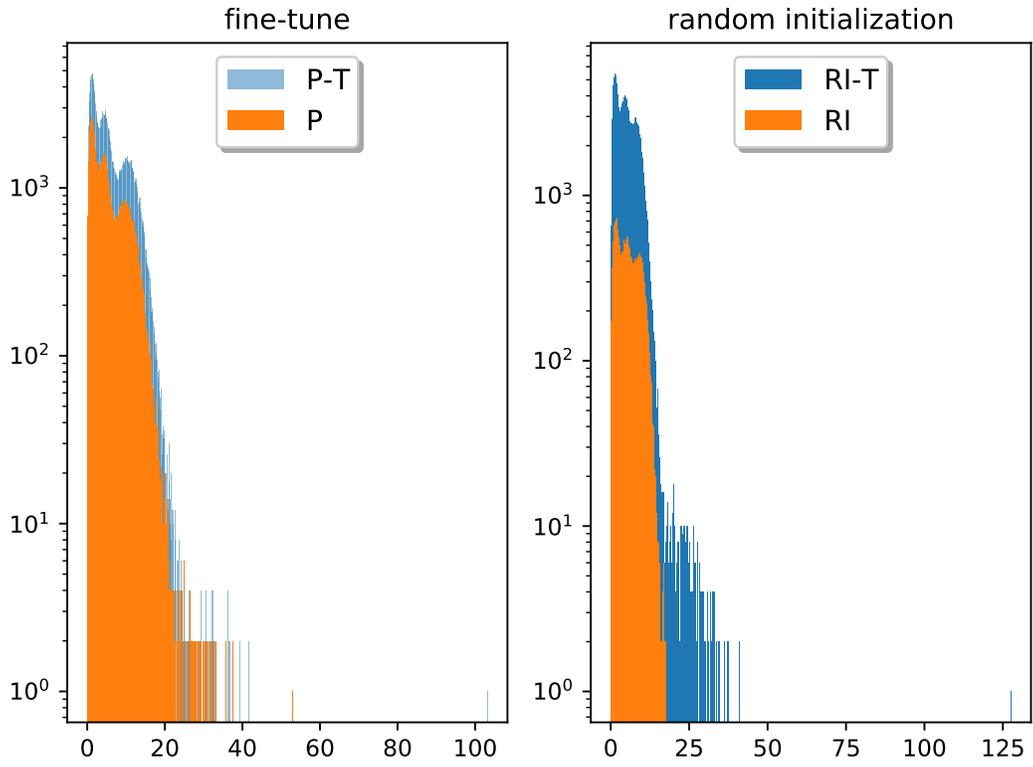

Figure 43: Spectrum Layer3.5 Conv2

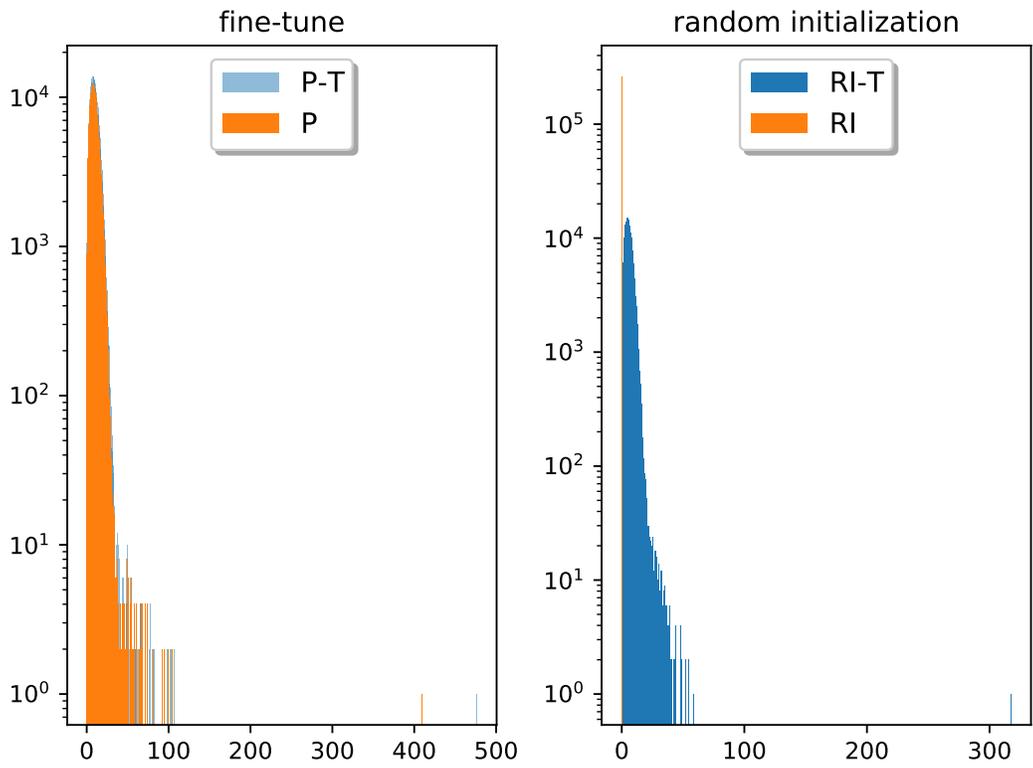

Figure 44: Spectrum Layer3.5 Conv3

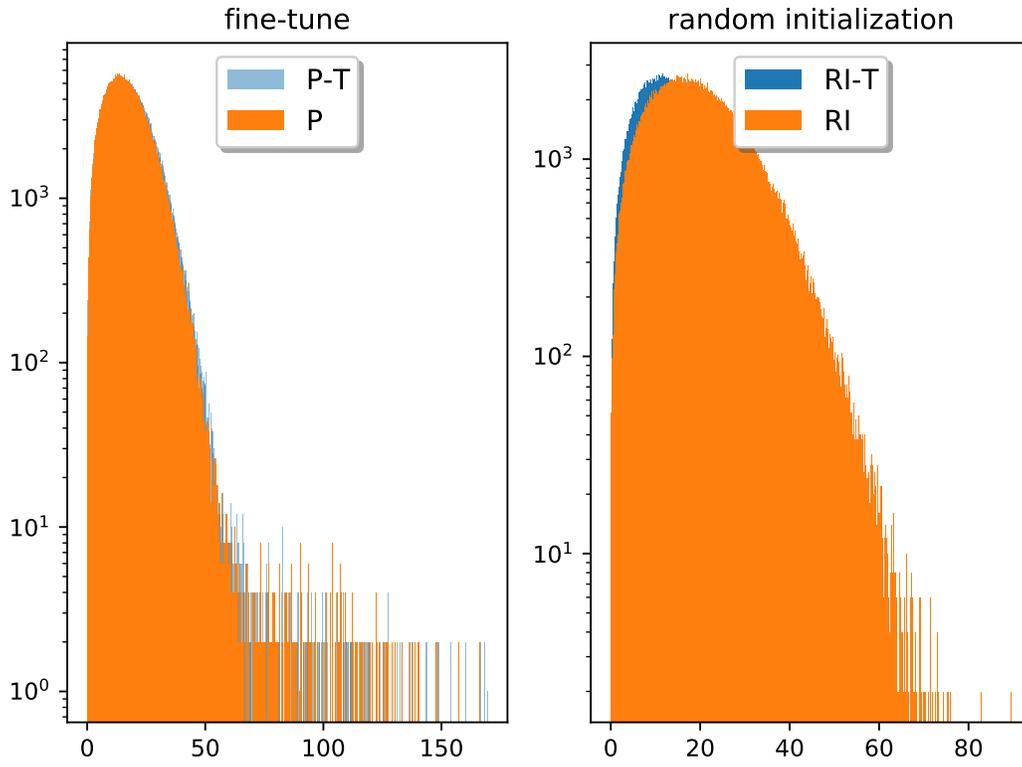

Figure 45: Spectrum Layer4.0 Conv1

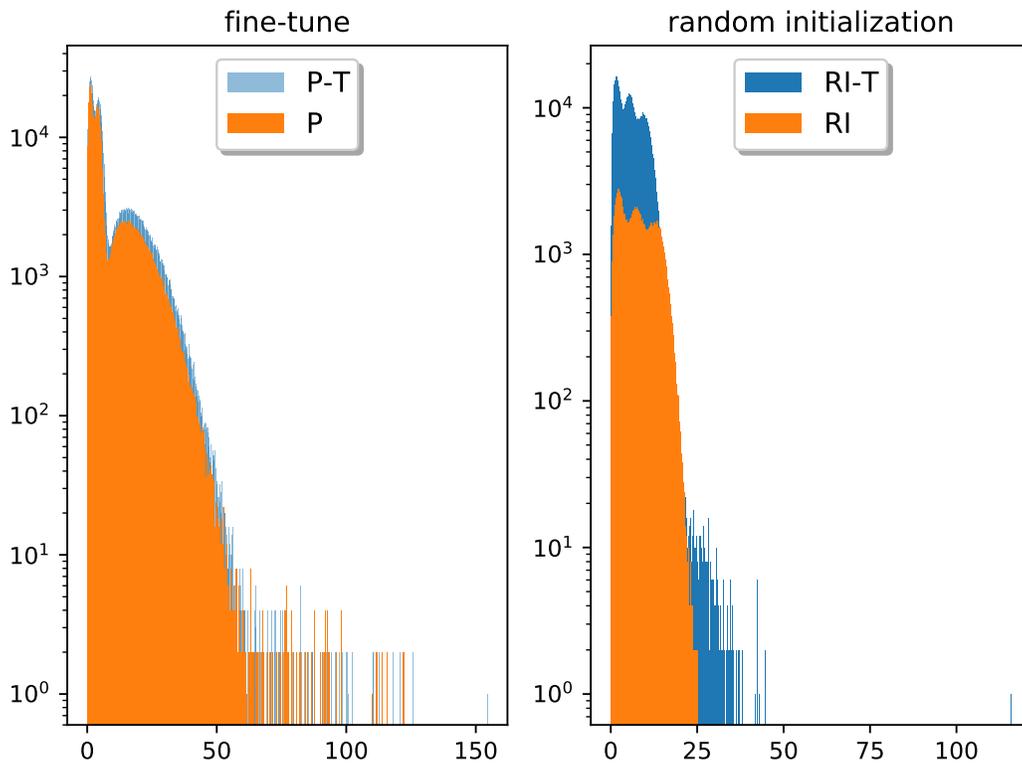

Figure 46: Spectrum Layer4.0 Conv2

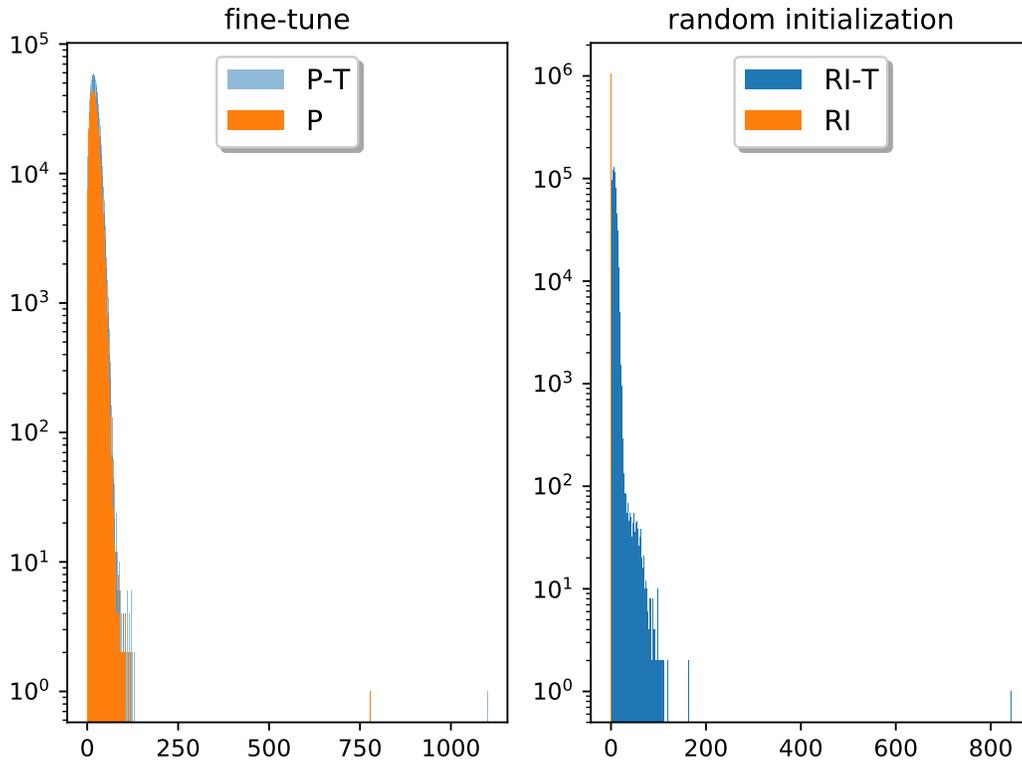

Figure 47: Spectrum Layer4.0 Conv3

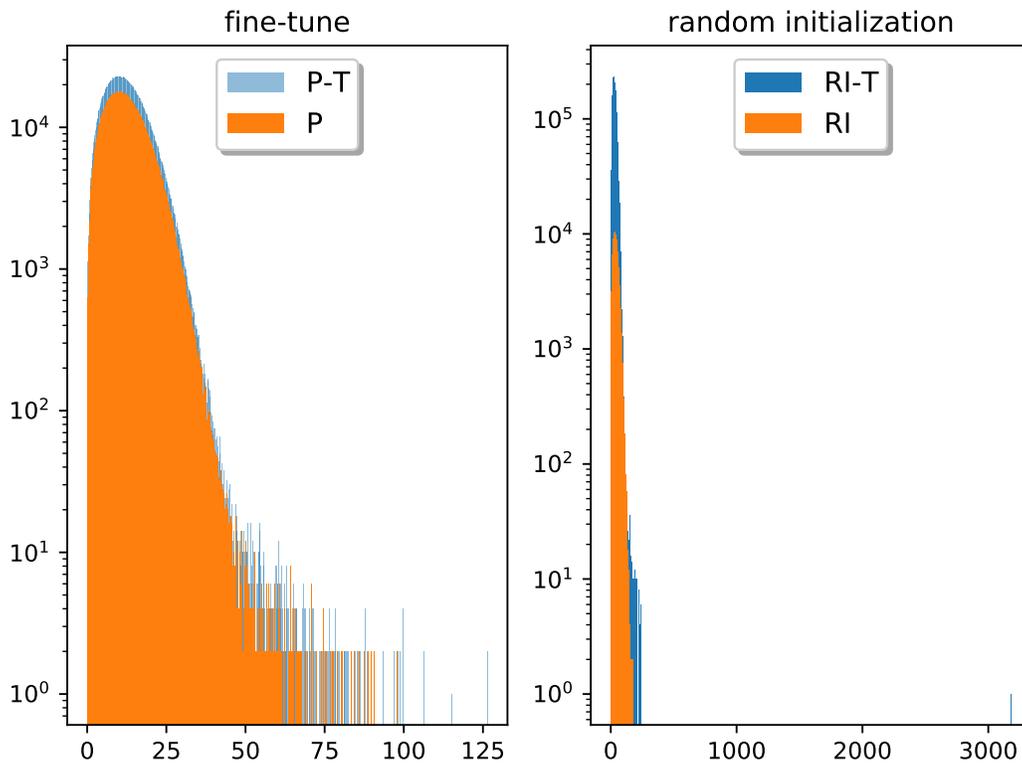

Figure 48: Spectrum Layer4.0 Downsample

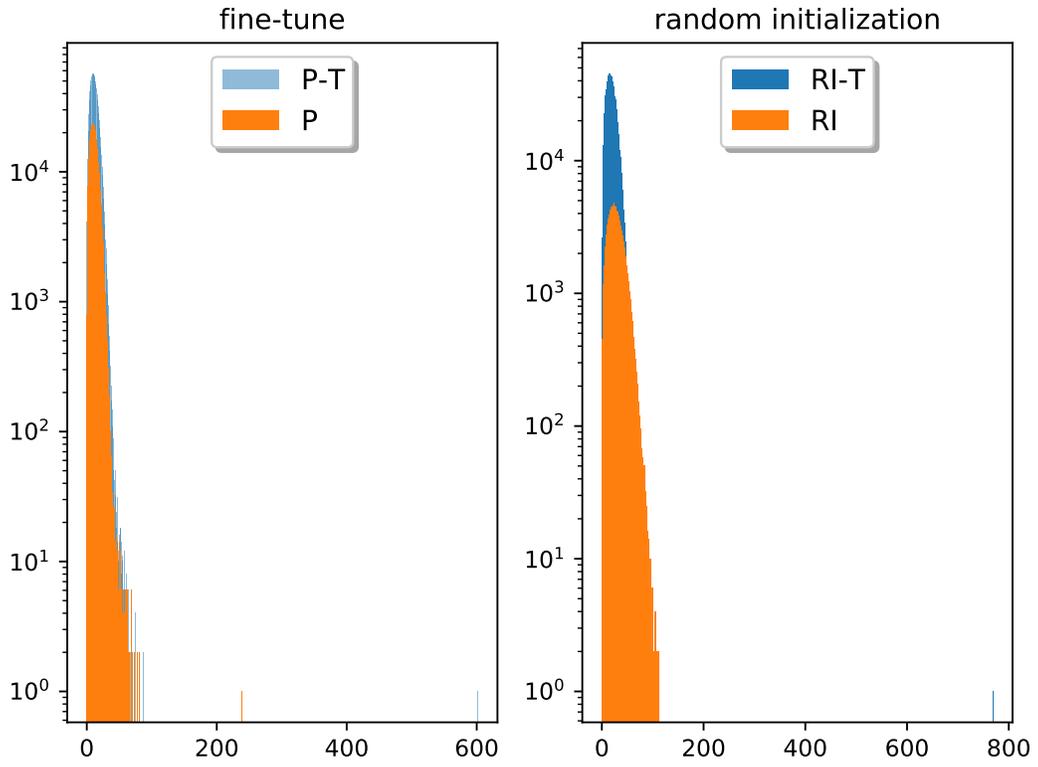

Figure 49: Spectrum Layer4.1 Conv1

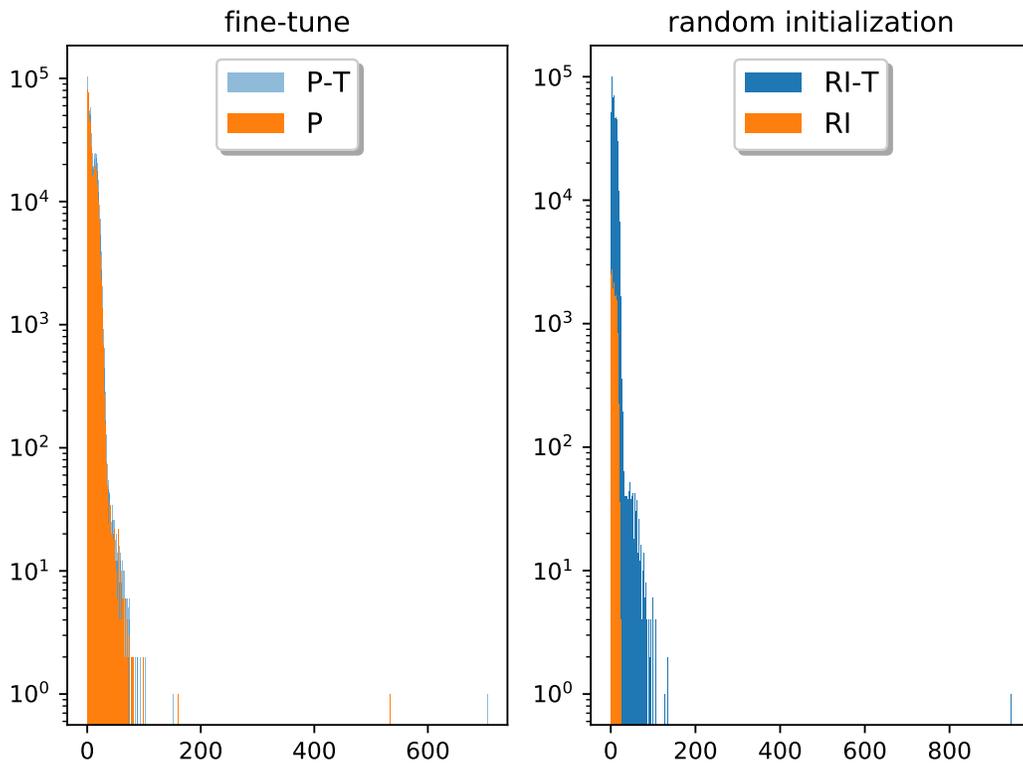

Figure 50: Spectrum Layer4.1 Conv2

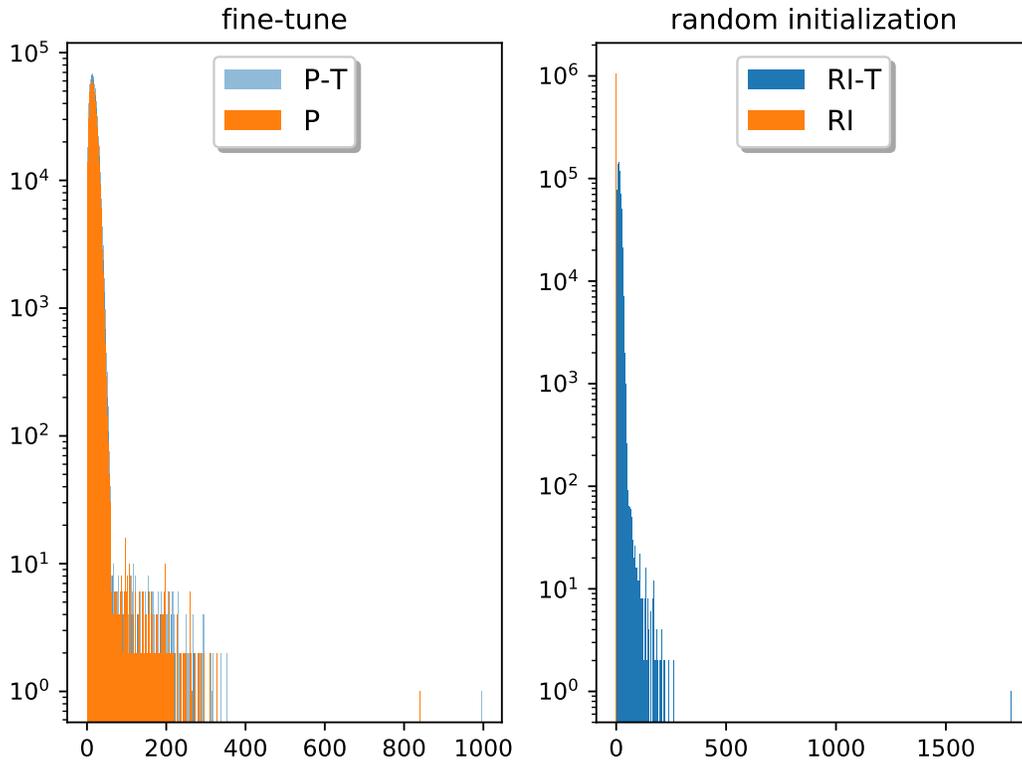

Figure 51: Spectrum Layer4.1 Conv3

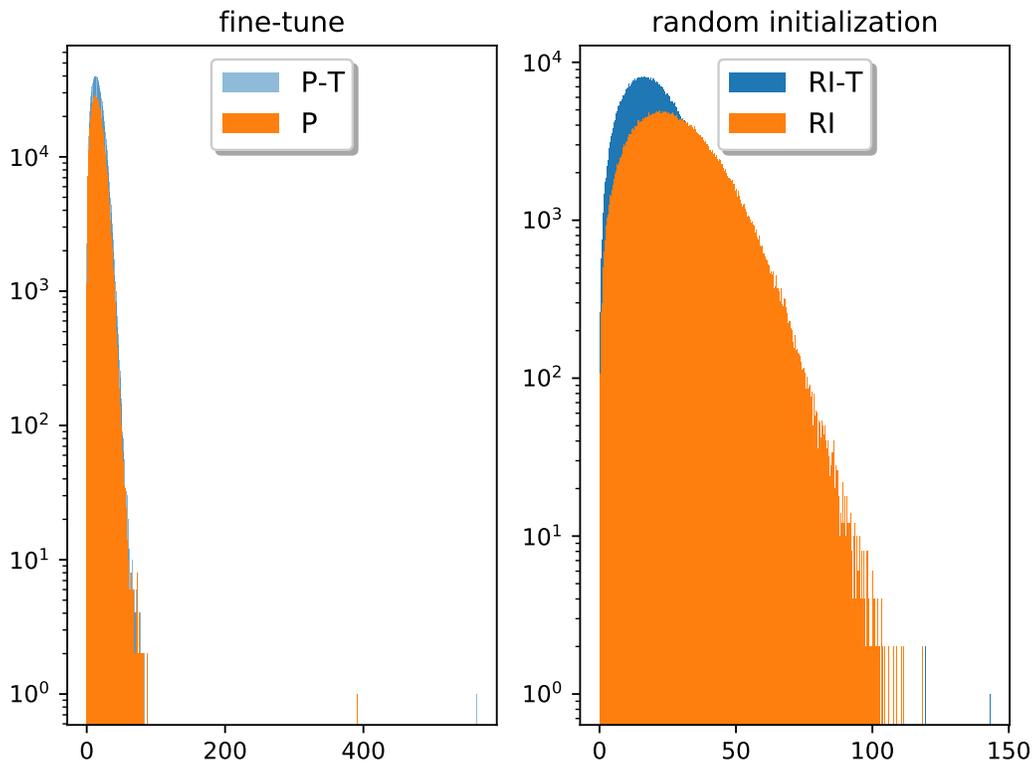

Figure 52: Spectrum Layer4.2 Conv1

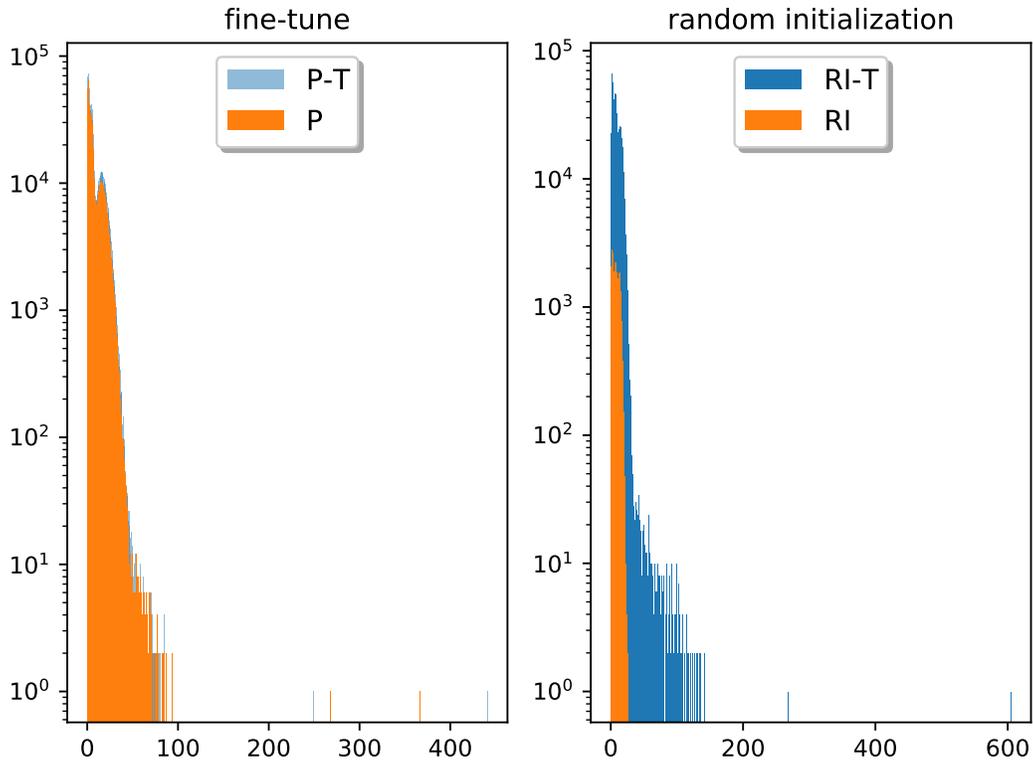

Figure 53: Spectrum Layer4.2 Conv2

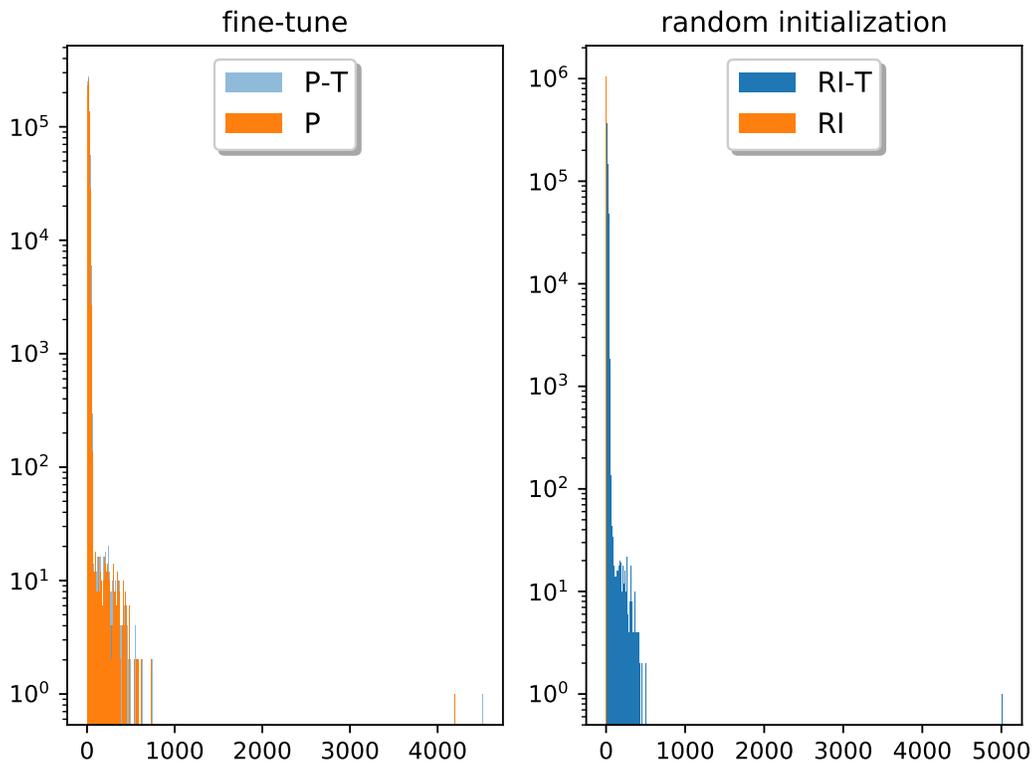

Figure 54: Spectrum Layer4.2 Conv3
